# Supplementary material for: High-Dimensional Geometric Streaming for Nearly Low Rank Data
Source: arXiv:2406.02910 source file (2024-06-05)
Supplement: Supplementary file 1 [file appendix.tex]

\onecolumn
\section{Construction of a Well-Conditioned Basis}\label{sec:proof-of-well-conditioned-basis}
\begin{definition}
Given an $n \times d$ matrix $A$, we call a matrix $U \in \R^{n \times d}$ an $(\alpha,\beta,p)$ well-conditioned basis for the column space of $A$ if all of the following hold:
\begin{enumerate}
	\item $U$ has the same column space as $A$,
	\item $\sum_{j \in [d]}\|U_{*j}\|_p^p = \sum_{i \in [n]}\|U_{i*}\|_p^p \le \alpha$, and
	\item for all vectors $x \in \R^{n \times d}$, we have $\|x\|_q \le \beta\|Ux\|_p$ where $1/q+1/p = 1$.
\end{enumerate}	
\end{definition}
\subsection{Construction using L\"owner-John Ellipsoids}
\begin{theorem}
	For all $n \times d$ matrices $A$, there exists a $(d,d^{\max(1-1/p, 1/2)} ,p)$ well-conditioned basis $U$ for the column space of $A$. Moreover, for all $x \in \R^d$,
	\begin{align*}
		\frac{1}{\sqrt{d}}\opnorm{x} \le \lp{Ux} \le \opnorm{x}.
	\end{align*}
	\label{thm:well-conditioned-basis}
\end{theorem}
We use the following L\"owner-John ellipsoid theorem, to prove the above theorem.
\begin{theorem}[L\"owner-John Ellipsoid Theorem]
	For any convex body $C \subseteq \R^n$ symmetric about the origin, there exists an ellipsoid $E := \setbuilder{x}{\T{x}Fx \le 1}$ for some positive semidefinite matrix $F$ satisfying
	\begin{align*}
		E \subseteq C \subseteq \sqrt{d}E.
	\end{align*}
	In particular, the ellipsoid of maximum volume that lies inside $C$ satisfies the above property.
\end{theorem}
\begin{proof}[Proof of Theorem~\ref{thm:well-conditioned-basis}]
Given a matrix $A$, consider the set $C_{A,p}$ defined as
\begin{align*}
	C_{A,p} := \setbuilder{x \in \R^d}{\|Ax\|_p \le 1}.
\end{align*}
It follows from the properties of the $\ell_p$ norm that $C_{A,p}$ is both convex and symmetric about the origin. From the L\"owner-John ellipsoid theorem, there exists an ellipsoid $E := \setbuilder{x}{\T{x}Fx \le 1}$ satisfying $E \subseteq C_{A,p} \subseteq \sqrt{d}E$. Now consider an arbitrary $x$ satisfying $\|Ax\|_p = 1$. By definition of $C_{A,p}$, the point $x$ lies on the boundary of the convex set $C_{A,p}$. As $ 0 \in E \subseteq C_{A,p}$, there exists an $\alpha \le 1$ such that $\alpha x$ lies on the boundary of the ellipsoid $E$ which implies that
\begin{align*}
	\T{(\alpha x)}F(\alpha x) = 1
\end{align*}
from which we have $\T{x}Fx = 1/\alpha^2\ge 1$. 
Similarly, as $C_{A,p} \subseteq \sqrt{d}E$, there exists a $\beta \ge 1$ for which $\beta x$ lies on the boundary of $\sqrt{d}E$ which implies $(\beta x/\sqrt{d})$ lies on the boundary of $E$ and that $\T{((\beta/\sqrt{d}) x)}F((\beta/\sqrt{d}) x) = 1$ which implies $\T{x}Fx = d/\beta^2 \le d$. 
Thus we have that for all $x$ such that $\|Ax\|_p = 1$,
\begin{align*}
	\|Ax\|_p \le \sqrt{\T{x}Fx} \le \sqrt{d}\|Ax\|_p.
\end{align*}
By the fact that $\|\alpha Ax\|_p = |\alpha|\|Ax\|_p$, we conclude that for all $x \in \R^d$, 
\begin{align*}
	\frac{1}{\sqrt{d}} \sqrt{\T{x}Fx} \le \|Ax\|_p \le \sqrt{\T{x}Fx}.
\end{align*}
Let $F = \T{G}G$ for some invertible matrix $G$ which exists as the matrix $F$ is positive definite if the matrix $A$ has full column rank. 
Then the above inequality implies that
$
	({1}/{\sqrt{d}})\opnorm{Gx} \le \|Ax\|_p \le \opnorm{Gx}
$ and therefore that for all $x \in \R^d$,
\begin{align*}
	\frac{1}{\sqrt{d}}\opnorm{x} = \frac{1}{\sqrt{d}}\opnorm{G (G^{-1}x)} \le \|A(G^{-1}x)\|_p \le \opnorm{G(G^{-1}x)} = \opnorm{x}.
\end{align*}
We now claim that $U := AG^{-1}$ is a well-conditioned basis for $A$. Clearly, the column space of $U$ is the same as the column space of $A$. We have
\begin{align*}
	\sum_{i \in  [d]}\|U_{*i}\|_p^p = \sum_{i \in [d]}\|Ue_i\|_p^p \le \sum_{i \in [d]}\|e_i\|_2^p = d
\end{align*}
and for any $x$,
\begin{align*}
	\|x\|_q \le d^{\max(1/q-1/2, 0)}\|x\|_2 \le d^{\max(1/q, 1/2)}\|Ux\|_p.
\end{align*}
Thus, $U$ is a $(d, d^{\max(1-1/p, 1/2)}, p)$ well-conditioned basis for $A$.	
\end{proof}

\subsection{Construction using Lewis weights}
Given a matrix $A$, the $\ell_p$ Lewis weights of $A$ are the \emph{unique} weights $w \in [0,1]^n$ satisfying
\begin{align*}
	w_i = \tau_i^{\ell_2}(\diag(w)^{1/2-1/p}A).
\end{align*}
See \cite{cohen2015lp} for an overview of Lewis weights and fast algorithms to compute approximations to Lewis weights.
Let $QR := \diag(w)^{1/2-1/p}A$ be the QR-decomposition and define $H := AR^{-1}$. It is shown in \cite{clarkson2019dimensionality,Lewis1978, wojtaszczyk1996banach} that the matrix $H$ has the following properties:
\begin{enumerate}
	\item For all $i \in [n]$, $\opnorm{H_{i*}} = w_i^{1/p}$, 
	\item $\diag(w)^{1/2-1/p}H = \diag(w)^{1/2-1/p}AR^{-1} = Q$ has orthonormal columns, and
	\item for all $x$,
	$
		\opnorm{x} \le \lp{Hx} \le d^{1/p-1/2}\opnorm{x}
	$
	when $p \le 2$, and
	$
		\lp{Hx} \le \opnorm{x} \le d^{1/2-1/p}\lp{Hx}
	$
	when $p \ge 2$.
\end{enumerate}
The properties imply that $H$ is a $(d,d^{1-2/p},p)$ well-conditioned basis for $p \ge 2$ and a $(d^{2-p/2},1,p)$ well-conditioned basis for $p \le 2$. Further, we have for all $i \in [n]$ and all $x \in \R^d$,
\begin{align}
	\frac{|(Hx)_{i}|}{\lp{Hx}} \le \frac{\opnorm{H_{i*}}\opnorm{x}}{\lp{Hx}} \le w_i^{1/p}d^{\max(1/2-1/p,0)}.
	\label{eqn:sensitivity-bound-lewis-weights}
\end{align}

\section{Subspace Embeddings via \texorpdfstring{$\ell_p$}{lp} sensitivity sampling}
\label{sec:lp-sensitivity-sampling}
\subsection{Offline Setting}
\begin{algorithm}
\caption{$\ell_p$ sensitivity sampling}	
\label{alg:lp-sensitivity-sampling}
\DontPrintSemicolon
\KwIn{$A \in \R^{n \times d}$, $p \ge 1$ and $v \in [0,1]^n$ satisfying $v_i \ge \beta\tau^{\ell_p}_{i}(A)$}
\KwOut{$\bS \in \R^n$}
For all $i \in [n]$, $p_i \gets \min(1, C_1\beta^{-1}v_i(C_2d\log(d) + \log(1/\delta))\varepsilon^{-2})$\;
$\bS \gets 0_{n \times n}$\;
\For{$i \in [n]$}{
	With probability $p_i$ set $\bS_{ii}$ to $(1/p_i)^{1/p}$\;
}
\Return{$\bS$}
\end{algorithm}

Given an $n \times d$ matrix $A$, the $\ell_p$ sensitivity of the $i$-th row $a_i$ is defined as
\begin{align*}
	\tau_i^{\ell_p}(A) := \max_x \frac{|\la a_i, x\ra|^p}{\lp{Ax}^p}.
\end{align*}
This is a straightforward extension of the $\ell_2$ leverage scores to the case of $p \ne 2$. Similar to how sampling rows with probabilities proportional to the $\ell_2$ leverage scores gives an $\ell_2$ subspace embedding \cite{drineas2006subspace}, we can show that sampling rows with probabilities proportional to the $\ell_p$ sensitivities gives $\ell_p$ subspace embeddings \cite{dasgupta2009sampling,clarkson2016fast}. The proof for $\ell_p$ regression using sensitivity sampling was first given in \cite{ken,dasgupta2009sampling}. 
%Using similar techniques, a proof for construction of $\ell_1$ subspace embeddings was given in a survey by \citet{woodruff2014sketching}. 
Here we state the result for constructions of $\ell_p$ subspace embeddings for all $p \ge 1$. The proof is similar to that of the $\ell_1$ subspace embedding construction in \cite{woodruff2014sketching}.
\begin{theorem}
	Given a matrix $A$ and a vector $v \in [0,1]^n$ such that for all $i \in [n]$, $v_i \ge \beta \tau_i^{\ell_p}(A)$ for some $\beta \le 1$, let a random diagonal matrix $\bS$ be generated as follows: for each $i \in [n]$ independently, set $\bS_{ii} = (1/p_i)^{1/p}$ with probability $p_i$ and $0$ otherwise. If $p_i \ge \min(1, C_1\beta^{-1}v_i(C_2d\log(d/\varepsilon) + \log(1/\delta))/\varepsilon^2)$ for large enough constants $C_1$ and $C_2$, then with probability $\ge 1 - \delta$, for all $x \in \R^d$,
	\begin{align*}
		\lp{\bS Ax} = (1 \pm \varepsilon)\lp{Ax}.
	\end{align*}
	\label{thm:sensitivity-sampling}
\end{theorem}
\begin{proof}
	Let $U$ be a $(d,d^{\max(1-1/p,1/2)},p)$ well-conditioned basis for the column space of $A$. Fix an arbitrary vector $x \in \R^d$ such that $\lp{Ux} = 1$. Define the random variables $\bX_i$ independently for $i \in [n]$ as follows:
	\begin{align*}
		\bX_i = \begin{cases}
				(1/p_i - 1)|U_{i*}x|^p & \text{with probability $p_i$}\\
					- |U_{i*}x|^p & \text{otherwise}.
				\end{cases}
	\end{align*}
	We have that $\sum_{i=1}^n \bX_i = \lp{\bS Ux}^p - \lp{Ux}^p$ and $\E[\bX_i] = 0$. We want to show that with a high probability, $|\sum_{i=1}^n \bX_i| \le p\varepsilon\lp{Ux}^p = p\varepsilon$.
	
	Consider two cases: $p_i = 1$ and $p_i < 1$. If $p_i = 1$, then $\bX_i = 0$ almost surely and therefore $\E[\bX_i^2] = 0$. If $p_i < 1$, then we have
	\begin{align*}
		|\bX_i| \le \frac{2}{p_i}|U_{i*}x|^p
	\end{align*}
	almost surely. Now, $|U_{i*}x|^p \le \tau_i^{\ell_p}(A)\lp{Ux}^p = \tau_i^{\ell_p}(A)$ by the definition of $\ell_p$ sensitivities. From the assumption that $p_i < 1$, we have $1 \ge p_i \ge C_1\beta^{-1}v_i(C_2d\log(d) + \log(1/\delta))\varepsilon^{-2}$. Thus,
	\begin{align*}
		|\bX_i| \le \frac{2}{p_i}\tau_i^{\ell_p}(A) \le \frac{2\varepsilon^2}{C_1\beta^{-1}v_i(C_2d\log(d)+\log(1/\delta))}\tau_i^{\ell_p} \le \frac{2\varepsilon^2}{C_1(C_2d\log(d) + \log(1/\delta))}
	\end{align*}
	as $\beta^{-1}v_i \ge \tau_i^{\ell_p}$. Thus, $\bX_i$ for $i \in [n]$ are all independent $0$ mean random variables and at most $2\varepsilon^2/C_1(C_2d\log(d) + \log(1/\delta))$ almost surely. We also have
	\begin{align*}
		\E[\bX_i^2] &= p_i(1/p_i - 1)^2|U_{i*}x|^{2p} + (1-p_i)|U_{i*}x|^{2p}\\
		&=(1-p_i)\frac{1}{p_i}|U_{i*}x|^{2p}\\
		&\le (1-p_i)\frac{1}{p_i}(\tau_i^{\ell_p}(A))|U_{i*}x|^p\\
		&\le \frac{\varepsilon^2}{C_1(C_2d\log(d)+\log(1/\delta))}|U_{i*}x|^p
	\end{align*}
	which implies $\sum_{i}\E[\bX_i^2] = (\varepsilon^2/C_1(C_2d\log(d) + \log(1/\delta)))\sum_{i:p_i \ne 1}|U_{i*}x|^p \le \varepsilon^2/C_1(C_2d\log(d)+\log(1/\delta))$. Using Bernstein's inequality, we obtain
	\begin{align*}
		\Pr[|\sum_{i=1}^n\bX_i| \ge p\varepsilon] &\le 2\exp\left(-\frac{p^2\varepsilon^2/2}{\varepsilon^2/C_1(C_2d\log(d) + \log(1/\delta)) + 2p\varepsilon^3/C_1(3C_2d\log(d) +3\log(1/\delta))}\right)\\
		&\le 2\exp\left(-\frac{p^2\varepsilon^2/2}{\varepsilon^2/C_1 + 2p\varepsilon^3/3C_1} (C_2d\log(d) + \log(1/\delta))\right).
	\end{align*}
	For $C_1 \ge (1+2p\varepsilon/3)/p^2$, we have 
	\begin{align*}
		\Pr[|\sum_i \bX_i| \ge p\varepsilon] \le 2\delta\exp(-C_2d\log(d)).
	\end{align*}
	Thus, for a fixed $x \in \R^d$ with $\lp{Ux} = 1$, we obtain that $\lp{\bS Ux} = (1 \pm 2\varepsilon)$ with probability $\ge 1 - 2\delta\exp(-C_2d\log(d/\varepsilon))$. We now use a net argument to show that $\lp{\bS Ux}$ approximates $\lp{Ux}$ for all $x$. 
	
	  Consider the set $K = \setbuilder{x}{\lp{Ux} = 1}$. As $(1/\sqrt{d})\opnorm{x} \le \lp{Ux}$, we obtain that the set $K$ is inside the $\ell_2$ ball of radius $\sqrt{d}$ in $\R^d$. Consider an $\varepsilon$ net $\calN \subseteq K$ satisfying the property that for every $x \in K$ there is a $y_x \in \calN$ satisfying
  \begin{align*}
      \opnorm{x - y_x} \le \varepsilon.
  \end{align*}
  A greedy construction of such a net $\calN$ shows that there exists an $\varepsilon$ net of $K$ of size $|\calN|$ at most $\exp(d\log(1+\sqrt{d}/\varepsilon)) \le \exp(5d\log (d/\varepsilon))$ (see e.g., \cite{dasgupta2009sampling}). Now by a union bound over all the vectors in $\calN$, we obtain that with a probability $\ge 1 - \delta$, for all $y \in \calN$,
  \begin{align*}
      \lp{\bS Uy} = (1 \pm \varepsilon).
  \end{align*}
Let $\eta := \max_{x \in K}|\lp{\bS Ux} - \lp{Ux}|$ and let $x^* \in K$ achieve the value $\eta$. As $\calN$ is an $\varepsilon$-net for $K$, we have that there is a vector $y \in K$ satisfying $\opnorm{x^* - y} \le \varepsilon$. Now,
\begin{align*}
    \eta = |\lp{\bL Ux^*} - 1|.
\end{align*}
Assume $\lp{\bS Ux^*} = 1 + \eta$. The other case proceeds similarly. By the triangle inequality, 
\begin{align*}
    \eta = \lp{\bS Ux^*} - 1 \le \lp{\bS Uy} + \lp{\bS U(x^* - y)} - 1.
\end{align*}
Note that $(x^* - y)/\lp{U(x^*- y )} \in K$ and therefore $\lp{\bS U(x^* - y)} \le (1+\eta)\lp{U(x^* - y)} \le (1 + \eta)\opnorm{x^* - y} \le \varepsilon(1+\eta)$. Here we used the fact that for all $x$, $\lp{Ux} \le \opnorm{x}$. Thus,
\begin{align*}
    \eta \le (\lp{\bS U y} - 1) + (1 + \eta)\varepsilon \le \varepsilon + (1 + \eta)\varepsilon
\end{align*}
and hence we obtain $\eta \le (2\varepsilon)/(1 - \varepsilon) \le 3\varepsilon$. Thus for all $x \in K$, 
\begin{align*}
    |\lp{\bS Ux} - 1| \le 3\varepsilon.
\end{align*} Picking $C_2 \ge 4$ is enough to ensure that the success probability $\ge 1 - \delta$. By scaling $\varepsilon$ appropriately, we obtain the result.
	\end{proof}

When given access to exact $\ell_p$ sensitivities of the rows, the sampling process in the above theorem (Algorithm~\ref{alg:lp-sensitivity-sampling}) samples, by using a Chernoff bound, $O((\sum_i \tau_i^{\ell_p}(A))(d\log(d) + \log(1/\delta))/\varepsilon^2)$ rows with high probability. By \eqref{eqn:sensitivity-bound-lewis-weights}, we have
	\begin{align*}
		\tau_i^{\ell_p}(A) = \max_x \frac{|\la a_i, x\ra|^p}{\lp{Ax}^p} \le w_i d^{\max(p/2-1,0)},
	\end{align*}
	where $w_i$ denotes the $i$-th $\ell_p$ Lewis weight of $A$. Using the fact that Lewis weights add up to at most $d$, we obtain that $\sum_{i}\tau_i^{\ell_p}(A) \le d^{\max(p/2,1)}$. Thus, the row sampling algorithm from Theorem~\ref{thm:sensitivity-sampling}, when given access to constant factor approximations of  $\ell_p$ sensitivities samples at most	$O(d^{\max(p/2+1,2)}\log(d)/\varepsilon^2)$ rows with high probability and outputs a subspace embedding with probability $\ge 1 - \exp(d\log d)$. Note that for $p=2$, it can be shown that sampling $O(d\log(d)/\varepsilon^2)$ rows suffices using a Matrix-Chernoff bound instead of the net argument in the proof of Theorem~\ref{thm:sensitivity-sampling}.
\subsection{Online Setting}
\begin{algorithm}
\caption{Online $\ell_p$ sensitivity sampling}
\label{alg:online-lp-sampling}
\DontPrintSemicolon
\KwIn{Rows $a_1,\ldots,a_n \in \R^d$ of an $n \times d$ matrix $A$ arriving in a stream, $p \ge 1$ and  $\varepsilon > 0$}
\KwOut{$\bS A$}
$\bS \gets 0_{n \times n}$\;
\For{$i \in [n]$}{
	$\tau_i^{\OL,\ell_p} \gets \max_x {|\angles{a_i, x}|^p}/{\lp{A_{1:i}x}^p}$\;
	$p_i \gets \min(1, C_1\tau_i^{\OL,\ell_p}(C_2d\log(d) + \log(n))\varepsilon^{-2})$\;
	With probability $p_i$, set $\bS_{ii}$ to $(1/p_i)^{1/p}$\;
}	
\Return{$\bS A$}
\end{algorithm}

	Consider an $n \times d$ matrix $A$ with rows $a_1,\ldots,a_n \in \R^d$ arriving in a stream. Let $\tau_i^{\OL,\ell_p}(A)$ be the \emph{online} $\ell_p$ sensitivity of the $i$-th row defined as
	\begin{align*}
		\tau_i^{\OL,\ell_p}(A) := \max_x \frac{|\la a_i, x\ra|^p}{\lp{A_{1:i}x}^p},
	\end{align*}
	where $A_{1:i}$ denotes the matrix formed by first $i$ rows of $A$. Clearly, $\tau_i^{\OL,\ell_p}(A) \ge \tau_i^{\ell_p}(A)$ for all $i \in [n]$ as $\lp{A_{1:i}x} \le \lp{Ax}$ with equality achieved at $i = n$. When rows of $i$ appear online, then the sampling process in Theorem~\ref{thm:sensitivity-sampling} (Algorithm~\ref{alg:lp-sensitivity-sampling}) can be run by using online $\ell_p$ sensitivities instead of offline $\ell_p$ sensitivities. As Theorem~\ref{thm:sensitivity-sampling} requires only an upper bound on the $\ell_p$ sensitivities, which is provided by the online $\ell_p$ sensitivities, the algorithm succeeds in constructing an $\ell_p$ subspace embedding for the matrix $A$.
	
	The algorithm samples $O((\sum_i \tau_i^{\OL, \ell_p}(A))(d\log(d) + \log(1/\delta))/\varepsilon^2)$ rows with high probability. Interestingly, it is possible to bound the sum of online $\ell_p$ sensitivities and show that for ``well-conditioned'' instances, it is not too large compared to the upper bound on the sum of offline $\ell_p$ sensitivities.
	
\begin{theorem}
	Given an $n \times d$ matrix $A$, let $\kappa^{\OL}$ be defined as
	\begin{align*}
		\kappa^{\OL} := \frac{\opnorm{A}}{\min_{i\in [n]} \sigma_{\min}(A_{1:i})},
	\end{align*}
	where $\sigma_{\min}(\cdot)$ denotes the \emph{smallest} non-zero singular value of a matrix. For $p \ge 2$,
	\begin{align*}
		\sum_{i=1}^n \tau_i^{\OL,\ell_p}(A) = O((d\log n\kappa^{\OL})^{p/2}\log n)
	\end{align*}
	and for $p < 2$,
	\begin{align*}
		\sum_{i=1}^n \tau_i^{\OL,\ell_p}(A) = O((d\log n\kappa^{\OL})\log n).
	\end{align*}
	\label{thm:sum-of-online-sensitivities}
\end{theorem}

The upper bound on the sum of online $\ell_p$ sensitivities extends the ideas from the proof of the upper bound on the sum of online $\ell_2$ sensitivities from \cite{cohen2016online} to all $p \ne 2$. The main idea here is that if the online sensitivity of a row is large, then it must span a new ``direction'' given that the minimum singular value of the prefix seen so far is not large. We argue that if the online $\ell_2$ sensitivities of all the rows are small, then the online $\ell_p$ sensitivities of all the rows are small as well. In the case when all online $\ell_2$ sensitivities are not small, we can show that only a few rows have large online $\ell_2$ sensitivities. By appropriately scaling down the rows that have large online $\ell_2$ sensitivities, we obtain that for all ``unscaled'' rows, the sum of online $\ell_p$ sensitivities is bounded and for the ``scaled'' rows we use induction to argue that the sum of their online $\ell_p$ sensitivities is small. The upper bound on online $\ell_1$ sensitivities was first shown using these ideas in \cite{braverman2020near}. Their bound readily extends to all $p \in [1,2]$. A slightly different proof is required for $p > 2$ which is given after the main statement of the online $\ell_p$ sensitivity sampling algorithm.

%\begin{theorem}[Sum of online sensitivities {\cite[Theorem~3.10]{woodruff2022high}}]
%Let $A \in \Z^{n \times d}$ be an integer matrix with entries bounded by $\poly(n)$. Let $2 < p < \infty$. Then,
%\begin{align*}
%	\sum_{i=1}^n \tau_{i}^{\OL,\ell_p}(A) = O((d\log n)^{p/2}\log n).
%\end{align*}
%If $A$ is a real matrix with condition number $\kappa$, then
%\begin{align*}
%	\sum_{i=1}^n \tau_{i}^{\OL,\ell_p} = O((d\log \kappa)^{p/2}\log n).
%\end{align*}
%\end{theorem}
%\textcolor{red}{Not clear if the proof in \cite{woodruff2022high} is correct for bounded entries. In the online whack-a-mole theorem, we don't have any lower bound on the factor we scale down a row by if its online leverage score is $\ge \alpha$. So we can't upper bound the number of rows we modify online.}

\begin{theorem}
	Given the rows of $A$ in a stream, Algorithm~\ref{alg:online-lp-sampling} returns a matrix $\bS A$ that has, with high probability, $O((d\log n\kappa^{\OL})^{\max(p/2,1)}\log n(d \log d + \log n)\varepsilon^{-2})$ non-zero rows and with probability $\ge 9/10$ satisfies for all $i \in [n]$ that for all $x \in \R^d$,
	\begin{align*}
		\lp{(\bS A)_{1:i}x} = (1 \pm \varepsilon)\lp{A_{1:i}x}.
	\end{align*}
\end{theorem}
\begin{proof}
	As discussed above, the online $\ell_p$ sensitivity of a row $a_i$ is always at least the offline $\ell_p$ sensitivity of $a_i$ with respect to any prefix matrix $A_{1:j}$ for $j\ge i$. Using a failure probability of $\delta=1/10n$ in Theorem~\ref{thm:sensitivity-sampling}, we can union bound over all $i \in [n]$, that Algorithm~\ref{alg:online-lp-sampling} succeeds in constructing an $\ell_p$ subspace embedding for all prefixes $A_{1:i}$.
\end{proof}
\subsection{Proof of upper bound on the sum of online sensitivities}
Given a matrix $A = a_1 \circ \cdots \circ a_n$, let $A_{1:i}$ denote the $i \times d$ matrix $a_1 \circ \cdots \circ a_i$. Recall that the online $\ell_p$ sensitivity of $a_i$ with respect to $A$ as follows:
\begin{align*}
	\tau_i^{\OL,\ell_p}(A) = \max_x \frac{|\la a_i, x\ra|^p}{\|A_{1:i}x\|_p^p}.
\end{align*}

\begin{theorem}[\cite{cohen2016online}]
Let $A$ be an arbitrary $n \times d$ matrix. Let $\lambda > 0$ and define $B = \lambda I_d$. Define $X = B \circ A$. From the above definition, we have that $\tau_{d+i}^{\OL, \ell_2}(X)$ denotes the online $\ell_2$ sensitivity of the row $a_i$ with respect to matrix $X$. Then,
\begin{align*}
	\sum_{i=1}^n\tau^{\OL,\ell_2}_{d+i}(X) \le Cd\log(1 + \opnorm{A}^2/\lambda^2).
\end{align*}
\end{theorem}
\begin{lemma}[Online Whack-a-mole]
Given an arbitrary $n \times d$ matrix $A$ and a matrix $B := \lambda I_d$ as in the above theorem, for any $\alpha \in (0,1)$, scaling down some rows of an arbitrary $n \times d$ matrix $A$ using a diagonal matrix $W$ satisfying $0\prec W \preceq I_n$ gives a matrix $X' = B \circ (W \cdot A)$ such that for all $i \in [n]$,
\begin{align*}
	\tau_{d+i}^{\OL, \ell_2}(X') \le \alpha.
\end{align*}
We also have 
\begin{align*}
	|\setbuilder{i}{W_{ii} < 1}| \le (C/\alpha)d\log(1 + \opnorm{A}^2/\lambda^2).
\end{align*}
\label{lma:online-whack-a-mole}	
\end{lemma}
\begin{proof}
	Start with $W_{ii}$ all being equal to $1$. Note that $\tau_{d+i}^{\OL,\ell_2}(X')$ does not depend on the values of $W_{jj}$ for $j > i$. We iteratively proceed from $i = 1,\ldots,n$ and set the values for $W_{ii}$. 
	If $\tau_{d+i}^{\OL,\ell_2}(X') \le \alpha$ we keep $W_{ii} = 1$ and proceed to $i+1$.  
	If $\tau_{d+i}^{\OL,\ell_2}(X') > \alpha$, we pick a suitable value $0 < W_{ii} < 1$ such that 
	\begin{align*}
		\tau_{d+i}^{\OL}(X') = \alpha.
	\end{align*}
	Note that such a $W_{ii}$ must exist because the online sensitivities are continuous and monotonically increasing in the weight $W_{ii}$.
	At the end of this process, let $S := \setbuilder{i}{W_{ii} < 1}$. 
	We have for all $i \in S$,
	\begin{align*}
		\tau_{d+i}^{\OL, \ell_2}(X') = \alpha.
	\end{align*}
Thus, $\alpha |S| \le \sum_{i=1}^n \tau_{d+i}^{\OL, \ell_2}(X') \le Cd\log(1 + \opnorm{WA}^2/\lambda^2)$ from the above theorem. 
As $\opnorm{W} \le 1$, we obtain that $|S| \le (C/\alpha)d\log(1 + \opnorm{A}^2/\lambda^2)$ for a large enough universal constant $C$.
\end{proof}
\begin{lemma}
	If $M$ is an arbitrary $N \times d$ matrix and $i \in [N]$ is an arbitrary index, then for $p \ge 2$,
	\begin{align*}
		\tau_i^{\ell_p}(M) \le (\tau_i^{\ell_2}(M))^{p/2}N^{p/2-1}.
	\end{align*}
	
\label{lma:l2-bound-to-lp-bound}
\end{lemma}
\begin{proof}
Recall
	\begin{align*}
		\tau_i^{\ell_p}(M) = \max_x \frac{|\la M_{i*}, x\ra|^p}{\|Mx\|_{p}^p}.
	\end{align*}
	By linearity, we can restrict $x$ in the above definition to only those vectors such that $\opnorm{Mx}=1$. We also have $|\la M_{i*}, x\ra|^2 \le \tau_i^{\ell_2}(M)\opnorm{Mx}^2$. Thus,
	\begin{align*}
		\tau_i^{\ell_p}(M) = \max_{x\, :\, \opnorm{Mx}=1}\frac{|\la M_{i*}, x\ra|^p}{\|Mx\|_p^p} \le \max_{x:\opnorm{Mx}=1}\frac{(\tau_{i}^{\ell_2}(M))^{p/2}}{\|Mx\|_p^p}.
	\end{align*}
	Further, $\|Mx\|_2 \le N^{1/2-1/p}\|Mx\|_p$ which implies $\|Mx\|_p^p \ge \opnorm{Mx}^p/N^{p/2-1}$ and
	\begin{align*}
		\tau_i^{\ell_p}(M) \le (\tau_i^{\ell_2}(M))^{p/2}N^{p/2-1}. & \qedhere
	\end{align*}
\end{proof}

\begin{lemma}
	Given a matrix $A$, if for all $i \in [n]$, $\tau_i^{\ell_2}(A) \le \alpha$, then for all $p \in [1,2]$ and all $i \in [n]$,
	\begin{align*}
		\tau_i^{\ell_p}(A) \le \alpha.
	\end{align*}
	\label{lma:p-less-than-2}
\end{lemma}
\begin{proof}
Let $p \in [1,2]$ be arbitrary. We have for any vector $z$ that
\begin{align*}
	\opnorm{z}^2 &= \sum_{i} z_i^2 = \sum_i |z_i|^p |z_i|^{2-p}\le \max_i |z_i|^{2-p} \lp{z}^p.
\end{align*}
Now,
\begin{align*}
	\tau_{i}^{\ell_p}(A) &= \max_{x:\opnorm{Ax}=1}\frac{|\angles{a_{i},x}|^p}{\lp{Ax}^p} \le \max_{x:\opnorm{Ax}=1} \left(\frac{|\angles{a_i, x}|^p}{\opnorm{Ax}^2} \max_{j}|\la a_j, x\ra|^{2-p}\right).
\end{align*}
By definition of the $\ell_2$ sensitivity, we have for all $j$ that $|\la a_j,x\ra|^2 \le \tau_j^{\ell_2}(A)\opnorm{Ax}^2 \le \alpha$. Thus, $\tau_i^{\ell_p}(A) \le \alpha$ for all $i$.
\end{proof}

We now bound $\sum_{i=1}^n \tau_{d + i}^{\OL, \ell_p}(X)$.
\begin{lemma}
	Let $A$ be an arbitrary $n \times d$ matrix with $\opnorm{A} \le U$ and $B$ be an $d \times d$ matrix as defined above. Let $X = B \circ A$. Then, for $p \ge 2$,
	\begin{align*}
		\sum_{i=1}^n\tau^{\OL, \ell_p}_{d+i}(X) \le \ceil{\log_2(n)}(4Cd\log(1+U^2/\lambda^2))^{p/2}.
	\end{align*}
	\label{lma:bound-on-joint-matrix}
\end{lemma}
\begin{proof}
The inequality clearly holds for $n \le d$ as the online $\ell_p$ sensitivity of each row is at most $1$. Let $n \ge d$ and assume that we proved the statement for all $n < m$. Now consider an arbitrary $m \times d$ matrix $A$ with $\opnorm{A} \le U$. We want to show that $\sum_{i=1}^m \tau_{d+i}^{\OL,\ell_p}(B \circ A) \le \ceil{\log_2(m)}(4Cd\log(1+U^2/\lambda^2))^{p/2}$.

By Lemma~\ref{lma:online-whack-a-mole}, we have that there is a weight matrix $W$ satisfying $0 \preceq W \preceq I$ such that $\tau_{d+i}^{\OL,\ell_2}(B \circ (W \cdot A)) \le \alpha$ for all $i \in [m]$ and $|\setbuilder{i \in [m]}{W_{ii} \ne 1}| \le (C/\alpha)d\log(1+U^2/\lambda^2)$. By picking \[\alpha = 2Cd\log(1+U^2/\lambda^2)/m,\] we have $|\setbuilder{i \in [m]}{W_{ii} \ne 1}| \le m/2$. Define $P := \setbuilder{i \in [m]}{W_{ii} = 1}$. For $i \in P$, let $C_{d+i} := B \circ (W \cdot A)_{1:i}$. We have the following relations between the online and offline $\ell_p$ sensitivities of various matrices we defined: for $i \in P$,
\begin{align*}
	\tau_{d+i}^{\OL, \ell_p}(B \circ A) \le \tau_{d+i}^{\OL, \ell_p}(B \circ (W \cdot A)) = \tau_{d+i}^{\OL, \ell_p}(C_{d+i}) = \tau_{d+i}^{\ell_p}(C_{d+i}).
\end{align*}
The first inequality follows from the fact that multiplying rows $j < i$ with $W_{jj} < 1$ can only increase the $i$-th online $\ell_p$ sensitivity. The first equality follows directly from the definition as truncating rows $j > i$ does not affect the online $\ell_p$ sensitivity of the $i$-th row. Finally, we have the last equality as for any matrix the online $\ell_p$ sensitivity of the last row is equal to the offline $\ell_p$ sensitivity. 

Now as seen above, for all $i$, we have $\tau_{d+i}^{\ell_2}(C_{d+i}) = \tau_{d+i}^{\OL, \ell_2}(B \circ (W \cdot A)) \le 2Cd\log(1+U^2/\lambda^2)/m$. Note that the matrix $C_{d+i}$ has $d+i$ rows. 

We now consider the case $p\ge 2$. From Lemma~\ref{lma:l2-bound-to-lp-bound}, we have 
\begin{align*}
	\tau_{d+i}^{\ell_p}(C_{d+i}) \le (2Cd\log(1+U^2/\lambda^2)/m)^{p/2} (d+i)^{p/2-1}.
\end{align*}
We assumed that $d \le m$ which implies
\begin{align*}
	\tau_{d+i}^{\ell_p}(C_{d+i}) \le \frac{(4Cd\log(1+U^2/\lambda^2))^{p/2}}{m}.
\end{align*}
Therefore for all $i \in P$, \[\tau_{d+i}^{\OL,\ell_p}(B \circ A) \le \tau_{d+i}^{\OL,\ell_p}(B \circ (W \cdot A)) = \tau_{d+i}^{\ell_p}(C_{d+i}) \le (4Cd\log(1+U^{2}/\lambda^2))^{p/2}/m.\]

Now consider $i \notin P$ and the matrix $A_{-P}$ formed by all the rows not in $P$. It is clear that $\opnorm{A_{-P}} \le \opnorm{A} \le U$ and that the online $\ell_p$ sensitivity of $a_i$ with respect to the matrix $B \circ A$ is at most the online $\ell_p$ sensitivity of $a_i$ with respect to the matrix $B \circ (A_{-P})$. Now the matrix $A_{-P}$ has at most $m/2$ rows and from the induction hypothesis we have that
\begin{align*}
	\sum_{i \notin P}\tau_{d+i}^{\OL, \ell_p}(B \circ A_{-P}) \le \ceil{\log_2(m/2)}(4Cd\log(1+U^{2}/\lambda^2))^{p/2}.
\end{align*}
Thus,
\begin{align*}
	\sum_i\tau_{d+i}^{\OL, \ell_p}(B \circ A) &\le \sum_{i\in P}\tau_{d+i}^{\OL, \ell_p}(B \circ A) + \sum_{i\notin P}\tau_{d+i}^{\OL, \ell_p}(B \circ A)\\
	&\le m \frac{(4Cd\log(1+U^2/\lambda^2))^{p/2}}{m} + \ceil{\log_2(m/2)}(4Cd\log(1+U^2/\lambda^2))\\
	&\le \ceil{\log_2(m)}(4Cd\log(1+U^2/\lambda^2))^{p/2}.
\end{align*}
We have the proof by induction.
\end{proof}
We finally bound $\sum_{i=1}^n \tau_i^{\OL,\ell_p}(A)$.
\begin{theorem}
	Given any matrix $A$, let 
$
	\kappa^{\OL} := \opnorm{A}/\min_{i \in [n]}\sigma_{\min}(A_{1:i}),
$
where $\sigma_{\min}$ denotes the minimum non-zero singular value. Then, for $p \ge 2$,
\begin{align*}
	\sum_{i \in [n]}\tau_i^{\OL,\ell_p}(A) = O((d\log n\kappa^{\OL})^{p/2}\log n).
\end{align*}
For $1 \le p \le 2$,
\begin{align*}
	\sum_{i\in [n]}\tau_i^{\OL,\ell_p}(A) = O(d\log n\kappa^{\OL}\log n).
\end{align*}
\label{thm:bound-on-sum-of-online-sensitivities}
\end{theorem}
\begin{proof}
First consider the case $p \ge 2$. Let $i \in [n]$ be a row such that $\tau_i^{\OL,\ell_p}(A) < 1$. By definition,
	\begin{align*}
		\tau_i^{\OL,\ell_p}(A) = \max_x \frac{|\la a_i, x\ra|^p}{\lp{A_{1:i}x}^p}.
	\end{align*}
Let $\sigma_{\min}(A_{1:i})$ be the minimum non-zero singular value of $A_{1:i}$. Clearly, a maximizer of the above objective is in the rowspace of $A_{1:i}$. For any $x \in \text{rowspace}(A_{1:i})$, we have
\begin{align*}
	\lp{A_{1:i}x}^p \ge \frac{1}{i^{p/2-1}}\opnorm{A_{1:i}x}^p \ge \frac{\sigma_{\min}(A_{1:i})^p}{i^{p/2-1}}\opnorm{x}^p \ge \frac{\sigma_{\min}(A_{1:i})^p}{i^{p/2-1}}\lp{x}^p.
\end{align*}
So, $\lp{(B \circ (A_{1:i}))x}^p = \lambda^p \lp{x}^p + \lp{A_{1:i}x}^p \le (1 + \lambda^pi^{p/2-1}/\sigma_{\min}(A_{1:i})^p)\lp{A_{1:i}x}^p$. If $\lambda \le \sigma_{\min}(A_{1:i})/\sqrt{i}$, then 
\begin{align*}
	\lp{(B \circ (A_{1:i}))x}^p \le 2\lp{A_{1:i}x}^p
\end{align*}
for all $x \in \text{rowspace}(A_{1:i})$. Thus,
\begin{align*}
	\tau_i^{\OL,\ell_p}(A) \le 2\tau_{d+i}^{\OL,\ell_p}(B \circ A).
\end{align*}
Thus we have for $p \ge 2$ that $\sum_{i=1}^n \tau_i^{\OL,\ell_p}(A) = O((d\log n\kappa^{\OL})^{p/2}\log n)$ using Lemma~\ref{lma:bound-on-joint-matrix}.

For the case $1 \le p \le 2$, the proof proceeds similarly to that of Lemma~4.7 of \citet{braverman2020near}. Lemma~\ref{lma:p-less-than-2} is the extension of their Lemma~4.6 and the rest of the proof extends similarly for all $p \in [1,2]$.
\end{proof}

%%%%%%%

\section{Missing Proofs from Section~\ref{sec:partition}}
\begin{proof}[Proof of Theorem~\ref{thm:partition-theorem}]
	Consider a run of online $\ell_p$ sensitivity sampling of rows of $A$ to construct an $\ell_p$ subspace embedding with $\varepsilon = 1/2$ and a success probability of $1-1/\poly(n)$. From the upper bound on the sum of online sensitivities of a matrix $A$, we obtain that with probability $\ge 9/10$, the online $\ell_p$ sensitivity sampling algorithm samples at most $r = O((d\log n\kappa^{\OL})^{\max(p/2,1)}(d\log d + \log n))$ rows and re-weights them appropriately to give a subspace embedding. 
	
	Let $M_i$ be the matrix constructed by the online sensitivity sampling algorithm after looking at row $i$. By a union bound over the success of online sensitivity sampling, we obtain that with probability $\ge 9/10$, for all $i \in [n]$ and for all $x \in \R^d$,
	\begin{align}
		\frac{1}{2}\lp{A_{1:i}x} \le \lp{M_ix} \le 2\lp{A_{1:i}x}.
		\label{eqn:embedding-guarantee}
	\end{align}
Let $P := \setbuilder{i}{M_i \ne M_{i-1}} \cup \set{n}$. We have $|P| \le O((d\log n\kappa^{\OL})^{\max(p/2,1)}(d\log d + \log n))$. Let $i_1 < i_2 < \dots < i_{|P|}$ be the elements in the set $P c$. Now consider $i \in [n]$ which satisfies $i_j < i < i_{j+1}$ for some $j$. By definition of the set $P$, we have $M_{i}=M_{i_j}$ and using \eqref{eqn:embedding-guarantee}, we obtain that for all $x$,
\begin{align*}
	\lp{A_{1:i_j}x} \ge \frac{1}{2}\lp{M_{i_j}x} = \frac{1}{2}\lp{M_i x} \ge \frac{1}{4}\lp{A_{1:i} x}
\end{align*}
which implies that for all $x \in \R^d$,
\begin{align*}
	\frac{1}{4}\lp{A_{1:i}x} \le \lp{A_{1:{i_j}}x} \le \lp{A_{1:i}x}.
\end{align*}
Thus, we have a set $P$ satisfying the condition.
\end{proof}
\section{Missing Details from Section~\ref{sec:embedding-without-duplicates}}
\subsection{Contraction}
\begin{lemma}
For any $x \in \R^n$, with probability $1 - \delta$, 
\begin{align*}
    \linf{\bD x} \ge \frac{\|x\|_1}{C_2(\log 1/\delta)^3\log n}
\end{align*}
$\bD$ is constructed as described above from a $O(\log(n) + \log(1/\delta))$-wise independent hash family.
\label{lma:linf-lowerbound}
\end{lemma}
\begin{proof}
    Let $x \in \R^n$ be an arbitrary vector with $\|x\|_1 = 1$. For $j \ge 0$, define
\begin{align*}
	T_j := \setbuilder{i}{|x_i| \in (1/2^{j+1}, 1/2^j]}
\end{align*}
and let $m_j := \sum_{i \in T_j}|x_i|$. We have
$
	\sum_{j=0}^{\infty}m_j = \|x\|_1 = 1
$
and $\sum_{j \ge 2\log n}m_j \le 1/n$. Thus, there exists $j^* \le 2\log n$ satisfying $m_{j*} \ge 1/4\log n$ which implies
\begin{align}
	|T_{j^*}| \frac{1}{2^{j^*}} \ge \frac{1}{4\log n} \implies |T_{j^*}| \ge \frac{2^{j^*}}{4\log n}.
	\label{eqn:lower-bound-on-bucket-size}
\end{align}
We have two cases: $|T_{j^*}| \le (\log 1/\delta)^2$ and $|T_{j^*}| \ge (\log 1/\delta)^2$. In the first case, we obtain $1/2^{j^*} \ge 1/(4(\log 1/\delta)^2\log n)$ which implies that there is a coordinate of absolute value at least $1/2^{j^*+1} \ge 1/(8(\log 1/\delta)^2\log n )$ in $x$. As each coordinate is scaled by at least $1$ by $\bD$, we have $\linf{\bD x} \ge 1/(8(\log 1/\delta)^2\log n)$ with probability $1$.

Now consider the case of $|T_{j^*}| \ge (\log 1/\delta)^2$. For $i \in T_{j^*}$, let $\bX_i = 1$ if $\bg(i) \ge 2^{j^*}/\poly_1(\log 1/\delta,\log n)$ and $0$ otherwise for a polynomial $\poly_1(\log 1/\delta,\log n)$ to be determined later. As the hash function $\bh$ is drawn from a $k$-wise independent hash family, we have that the random variables $(\bX_i)_{i \in T_{j^*}}$ are $k$-wise independent and for each $i$,
\begin{align}
	\Pr[\bX_i=1] \ge \min\left(1, \frac{\poly_1(\log 1/\delta,\log n)}{2^{j^{*}+2}}\right)
	\label{eqn:success-probability-of-each-coordinate}
\end{align}
Again, if $2^{j^*} \le 8\poly_1(\log 1/\delta,\log n)$, we have $\linf{\bD x} \ge 1/(16\poly_1(\log 1/\delta,\log n))$ with probability $1$. So we assume, $2^{j^*} > 8\poly_1(\log 1/\delta,\log n)$. We have using \eqref{eqn:lower-bound-on-bucket-size} and \eqref{eqn:success-probability-of-each-coordinate}
\begin{align*}
	\mu := \sum_{i \in T_{j^*}}\E[\bX_i] \ge \frac{\poly_1(\log 1/\delta,\log n)}{2^{j^*+2}}|T_{j^*}| \ge \frac{\poly_1(\log 1/\delta,\log n)}{16\log n}
\end{align*}
and let
\begin{align*}
	\sigma^2 := \sum_{i \in T_{j^*}}\Var[\bX_i^2] = |T_{j^*}|\Pr[\bX_i = 1](1 - \Pr[\bX_i = 1]).
\end{align*}
We have $\sigma^2 \ge \poly_1(\log 1/\delta,\log n)/25\log n$ and $\sigma^2 \le 2\poly_1(\log 1/\delta,\log n)$ using the fact that $|T_{j^*}| \le 2^{j^*+1}$. We now use the following tail inequality for $k$-wise independent random variables.
\begin{theorem}[{\cite[Theorem~4]{schmidt1995chernoff}}]
	Let $\bX_1,\ldots,\bX_n$ be a sequence of $k$-wise independent random variables that satisfy $|\bX_i - \E[\bX_i]| \le 1$. Let $\bX = \sum_i \bX_i$ with $\E[\bX] = \mu$ and let $\sigma^2[\bX]$ be the variance of $\bX$ so that $\sigma^2[\bX] = \sum_{i=1}^n \sigma^2[\bX_i]$ (provided $k \ge 2$). Then for any even $k \le 3(\sigma^2[\bX])^{1/3}$,
	\begin{align*}
		\Pr[|\bX - \mu| \ge T] \le 2(k\sigma^2[\bX]/eT^2)^{k/2}.
	\end{align*}
\end{theorem}
We apply the above theorem for random variables $(\bX_i)_{i \in T_j^*}$ with $T = \mu/2$. We obtain,
\begin{align*}
	\Pr[\bX = 0] \le \Pr[|\bX - \mu| \ge \mu/2] \le 2\left(\frac{Ck\poly_1(\log 1/\delta,\log n)}{e\poly_1(\log 1/\delta,\log n)^2}\right)^{k/2}
\end{align*}
as long as $k \le 3(\poly_1(\log 1/\delta,\log n)/25\log n)^{1/3}$.

We set $k = C_1(\log(1/\delta))$, $\poly_1(\log 1/\delta,\log n) = 8C_1^3(\log (1/\delta))^3(\log n)$ and obtain that $\Pr[\bX = 0] \le \delta$. Thus, with probability $\ge 1 - \delta$, at least one of the random variables $(\bX_i)_{i \in T_{j^*}}$ is $1$, which implies that 
\[\linf{\bD x}  \ge \frac{2^{j*}}{\poly_1(\log 1/\delta,\log n)}\cdot{\frac{1}{2^{j^*+1}}} \ge \frac{1}{C_2(\log 1/\delta)^3\log n}.\]
Overall, for any vector $x \in \R^n$ with $\|x\|_1 = 1$, with probability $\ge 1 - \delta$,
\begin{align*}
	\linf{\bD x} \ge \frac{1}{2\poly_1(\log 1/\delta,\log n)} \ge \frac{1}{C_2(\log 1/\delta)^3\log n}
\end{align*}
for a constant $C_2$ large enough.
\end{proof}
\subsection{Dilation}
We now prove that for any $n \times d$ matrix, with a large probability, for all vectors $x$, $\linf{\bD^{1/p}Ax}$ is not too large compared to $\lp{Ax}$.
\begin{lemma}
For any matrix $A \in \R^{n \times d}$, with probability $\ge 1 - \delta$ over the hash function $\bh$, for all $x \in \R^d$,
\begin{align*}
    \linf{\bD^{1/p}Ax} \le \frac{d^{\max(1,1/2+1/p)}(\log n)^{1/p}}{\delta^{1/p}}\lp{Ax}.
\end{align*}
\label{lma:linf-upperbound}
\end{lemma}
\begin{proof}
Let $U$ be an $(\alpha,\beta,p)$ well-conditioned basis for the column space of $A$ obtained using the L\"owner-John ellipsoid. Let $\bD$ be the random matrix constructed as described above. We have for any $x$,
\begin{align*}
    \linf{\bD^{1/p}Ux} &\le \sum_{j \in [d]}\linf{\bD^{1/p}U_{*j}}|x_j|\\
    &\le (\sum_{j \in [d]}\linf{\bD^{1/p}U_{*j}}^p)^{1/p}\|x\|_q \le \beta(\sum_{j \in [d]}\linf{\bD^{1/p}U_{*j}}^p)^{1/p}\lp{Ux}.
\end{align*}
Here we first use the triangle inequality of $\linf{\cdot}$ norm, then apply H\"older's inequality and finally use the fact that $U$ is an $(\alpha,\beta,p)$ well-conditioned basis.
Now, we upper bound $\sum_{j \in [d]}\linf{\bD^{1/p}U_{*j}}^p$. We have
\begin{align*}
    \E[\linf{\bD^{1/p}U_{*j}}^p] &\le \E[\lp{\bD^{1/p}U_{*j}}^p]\\
    &= \sum_{i \in [n]}\E[\bD_{ii} U_{ij}^p]\\
    &\le \sum_{i \in [n]}U_{ij}^p\log n,
\end{align*}
since $\E[\bD_{ii}] = (\sum_{q=0}^{r-1}2^{q} \cdot (1/2^{q+1})) + 2^r \cdot (1/2^r) = r/2+1 =(\log_2 n)/2 + 1$. Thus, \[\E[\sum_{j \in [d]}\linf{\bD^{1/p}U_{*j}}^p] \le \sum_{i,j}U_{ij}^p\log(n) \le \alpha\log n.\] With probability $\ge 1 - \delta$, $\sum_{j \in [d]}\linf{\bD^{1/p}U_{*j}}^p \le (\alpha\log n)/\delta$ by Markov's inequality. Thus, with probability $\ge 1 - \delta$ over the hash function $\bh$, for all $x$,
\begin{align*}
    \linf{\bD^{1/p}Ux} \le \frac{\beta(\alpha \log n)^{1/p}}{\delta^{1/p}}\lp{Ux}.
\end{align*}
Using the fact that $\alpha = d$ and $\beta = d^{\max(1-1/p, 1/2)}$, we obtain that with probability $\ge 1 - \delta$,
\[\linf{\bD^{1/p}Ux} \le d^{\max(1,1/2+1/p)}(\log n)^{1/p}\lp{Ux}/\delta^{1/p}. \qedhere\]
\end{proof}
\subsection{Wrap-up}
\begin{proof}[Proof of Theorem~\ref{thm:lp-to-linf-embedding}]
    Let $U$ be the $(\alpha,\beta,p)$ well-conditioned basis for $A$ constructed using a L\"owner-John ellipsoid and let $\Lambda := \setbuilder{x}{\lp{Ux} = 1}$. We have that the set $\Lambda$ is contained in the $\ell_2$ ball of radius $\sqrt{d}$ in $\R^d$ as $\opnorm{x} \le \sqrt{d}\lp{Ux}$ for all $x$. Let $x \in \Lambda$ be arbitrary. 

Now,
$
    \linf{\bD^{1/p}Ux}^p = \linf{\bD z}
$
where $z \in \R^n$ is defined as $z_i = |U_{i*}x|^p$. As $\lp{Ux} = 1$, we have $\|z\|_1 = 1$. Thus by Lemma~\ref{lma:linf-lowerbound}, with probability $1 - \delta$,
\begin{align*}
    \linf{\bD^{1/p}Ux}^p = \linf{\bD z} \ge \frac{1}{C_2(\log 1/\delta)^3\log n}.
\end{align*}
Let $N \subseteq \Lambda$ be a $1/n^5$ net for $\Lambda$ i.e., for all $x \in \Lambda$, there exists $y_x \in N$ satisfying
\begin{align*}
    \opnorm{x - y_x} \le \frac{1}{n^5}.
\end{align*}
As $\Lambda$ lies in the $\ell_2$ ball of radius $\sqrt{d}$, we have $|N| \le \exp(d\log(1+\sqrt{d}n^5)) \le \exp(6d\log n)$. Upper bounds on net sizes are standard; see \cite{rudelson2010non} for a proof. We now union bound over all net vectors $y \in N$ and obtain that with probability $\ge 1 - \delta$ (by setting a failure probability of $\delta/\exp(6d\log n)$ for each vector), for all $y \in N$,
\begin{align*}
    \linf{\bD^{1/p}Uy} \ge \frac{1}{(C_2((d\log n)^3 + (\log 1/\delta)^3)\log n)^{1/p}}.
\end{align*}
We also condition on $\bD$ satisfying the property in Lemma~\ref{lma:linf-upperbound}. Now, let $x$ be any vector in the set $\Lambda$. We have
\begin{align*}
    \linf{\bD^{1/p}Ux} &\ge \linf{\bD^{1/p}Uy_x} - \linf{\bD^{1/p}U(x-y_x)}\\
                       &\ge \frac{1}{(C_2((d\log n)^3 + (\log 1/\delta)^3)\log n)^{1/p}} - \frac{d^{\max(1,1/2+1/p)}(\log n)^{1/p}}{\delta^{1/p}}\lp{U(x-y_x)}\\
                       &\ge \frac{1}{(C_2((d\log n)^3 + (\log 1/\delta)^3)\log n)^{1/p}} - \frac{d^{\max(1,1/2+1/p)}(\log n)^{1/p}}{\delta^{1/p}n^5}.
\end{align*}    
Here we used the property of the well-conditioned basis $U$ that $\lp{Ux} \le \opnorm{x}$ for all $x$ and $\opnorm{x-y_x} \le 1/n^5$ by construction of the net. If $\delta \ge 1/n$,  we obtain
\begin{align*}
    \linf{\bD^{1/p}Ux} \ge \frac{1}{2(C_2((d\log n)^3 + (\log 1/\delta)^3)\log n)^{1/p}}.
\end{align*}
Thus, with probability $\ge 1 - 2\delta$, we have that for all $x$,
\begin{align*}
    \frac{\lp{Ux}}{2(C_2((d\log n)^3 + (\log 1/\delta)^3)\log n)^{1/p}} \le \linf{\bD^{1/p}Ux} \le \frac{d^{\max(1,1/2+1/p)}(\log n)^{1/p}}{\delta^{1/p}}\lp{Ux}. & \qedhere
\end{align*}
\end{proof}
\section{Missing Proofs from Section~\ref{sec:deduplicated-embedding}}
\begin{proof}[Proof of Lemma~\ref{lma:upper-and-lower-bounds}]
	Let $P$ be the set obtained from Theorem~\ref{thm:partition-theorem} for the matrix $A$. Now, by setting the failure probability $\delta = \delta'/(2|P|)$ in Theorem~\ref{thm:lp-to-linf-embedding}, using a union bound, we have that with probability $\ge 1-\delta'$, for all $i_j \in P$ and for all $x \in \R^d$,
\begin{align*}
	\frac{\lp{A_{1:i_j}x}}{2(C_2((d\log n)^3 + (\log 2|P|/\delta')^3)\log n)^{1/p}} \le \linf{\bD_{1:i_j}^{1/p}A_{1:i_j}x}\le Cd^{\max(1,0.5+1/p)}(|P|/\delta')^{1/p}/\lp{A_{1:i_j}x}
\end{align*}
and
\begin{align*}
	\frac{\lp{A_{1:i_j-1}x}}{2(C_2((d\log n)^3 + (\log 2|P|/\delta')^3)\log n)^{1/p}} \le \linf{\bD_{1:i_j-1}^{1/p}A_{1:i_j-1}x}\le Cd^{\max(1,0.5+1/p)}(|P|/\delta')^{1/p}\lp{A_{1:i_j-1}x}.
\end{align*}

Using the fact that $|P| = O((d\log n\kappa^{\OL})^{\max(p/2,1)}(d\log d + \log n))$, we have from the above that for all $i_j \in P$ and $x \in \R^d$,
\begin{align}
	\frac{\lp{A_{1:i_j}x}}{d^{3/p}\poly(\log n, \log \kappa^{\OL}, \log 1/\delta')} \le \linf{\bD_{{1:i_j}}^{1/p}A_{1:i_j}x} \le \frac{d^{\max(1.5+1/p,0.5+3/p)}\poly(\log \kappa^{\OL}, \log n)}{(\delta')^{1/p}}\lp{A_{1:i_j}x}.
\label{eqn:in-the-partition}
\end{align}
and
\begin{align*}
	\frac{\lp{A_{1:i_j-1}x}}{d^{3/p}\poly(\log n, \log \kappa^{\OL}, \log 1/\delta')} \le \linf{\bD_{{1:i_j-1}}^{1/p}A_{1:i_j-1}x} \le \frac{d^{\max(1.5+1/p,0.5+3/p)}\poly(\log \kappa^{\OL}, \log n)}{(\delta')^{1/p}}\lp{A_{1:i_j-1}x}.  
\end{align*}
Using the properties of $P$, we now show that a similar guarantee extends to all $i \in [n]$ instead of just $i_j \in P$. Consider an arbitrary $i \in [n] - P$ such that $i_j < i \le i_{j+1}-1$. We first note the following relations:
\begin{enumerate}
	\item For all $x \in \R^d$,
	\begin{align*}
		\linf{\bD_{{1:i_j}}^{1/p}A_{1:i_j}x} \le \linf{\bD_{{1:i}}^{1/p}A_{1:i}x} \le \linf{\bD_{1:i_{j+1}-1}^{1/p}A_{1:i_{j+1}-1}x}.
	\end{align*}
	\item For all $x \in \R^d$, by Theorem~\ref{thm:partition-theorem},
	\begin{align*}
		\lp{A_{1:i_j}x} \le \lp{A_{1:i}x} \le 4\lp{A_{1:i_j}x}
	\end{align*}
 and
 \begin{align*}
     \lp{A_{1:i}x} \le \lp{A_{1:i_{j+1}-1}x} \le 4\lp{A_{1:i}x}.
 \end{align*}
\end{enumerate}
First, we have
\begin{align}
	\linf{\bD_{{1:i}}^{1/p}A_{1:i}x} \ge \linf{\bD_{{1:i_j}}^{1/p}A_{1:i_j}x} \ge \frac{\lp{A_{1:i_j}x}}{C(d^3\log^4 n\log\log \kappa^{\OL})^{1/p}} \ge \frac{\lp{A_{1:i}x}}{4C(d^3\log^4 n\log\log \kappa^{\OL})^{1/p}}
	\label{eqn:outside-partition-1}
\end{align}
and
\begin{align}
	\linf{\bD_{{1:i}}^{1/p}A_{1:i}x} \le \linf{\bD_{{1:i_{j+1}-1}}^{1/p}A_{1:i_{j+1}-1}x} &\le Cd^{\max(1.5+1/p,0.5+3/p)}\poly(\log \kappa^{\OL}, \log n)\lp{A_{1:i_{j+1}-1}x}\nonumber\\
 &\le 4Cd^{\max(1.5+1/p,0.5+3/p)}\poly(\log \kappa^{\OL}, \log n)\lp{A_{1:i}x}.
	\label{eqn:outside-partition-2}
\end{align}
\end{proof}
\begin{proof}[Proof of Theorem~\ref{thm:main-theorem}]
Fix the $n \times d$ matrix seen in the stream. Let $H$  be an $O(d\log n + (p/2)(\log d + \log\log n + \log\log \kappa^{\OL}(B)))$-wise independent family of hash functions from $[N] \rightarrow [N]$. Let $\bh \sim H$ be a uniform random hash function and for all $i$. Let $\bD_{ii} = \bg(t_i)$, where $\bg$ is as defined in \eqref{eqn:definition-of-g}. Note that if $t_i = t_j$, then $\bD_{ii} = \bD_{jj}$. Let $M = \set{t_1,\ldots,t_n}$ denote the set of tags and let $|M| = m$. Let $t'_1, t'_2,\ldots,t'_m$ be the tags in the order they first appear in the stream.

Let $B \in \R^{m \times d}$ be the matrix formed by rows in the stream that correspond to distinct tags and let the order of the rows in the matrix $B$ be determined by the order in which the tags first appear in the stream. For any prefix $B_{1:i}$ of matrix $B$, let $\bD|_{B_{1:i}}$ denote the sub-matrix of $\bD$ formed by the rows that correspond to the first $i$ distinct tags in the stream. Thus we have $\bD|_B = \bD|_{B_{1:m}}$ is formed by the hash values of distinct tags. We condition on the matrix $\bD|_{B}$ satisfying the conditions in Lemma~\ref{lma:upper-and-lower-bounds}.

Let $S_i$ be the subset of rows maintained by the deterministic algorithm (Algorithm~\ref{alg:l-infinity-coreset}) after streaming until the $i$-th element $(a_i,t_i)$ in the stream. We abuse notation and also use $S_i$ to denote the matrix which selects the rows corresponding to the set $S_i$. Now, we have the guarantee that for all $x$,
\begin{align*}
	\linf{S_i \bD_{1:i}^{1/p}A_{1:i}x} \le \linf{\bD_{1:i}^{1/p}A_{1:i}x} \le O(\sqrt{T})\linf{S_i \bD_{1:i}^{1/p}A_{1:i}x},
\end{align*}
where $T$ is an upper bound on the sum of online $\ell_2$ sensitivities of the matrix $\bD^{1/p} A$.
Here $S_i\bD_{1:i}^{1/p}A_{1:i}$ is just the subset of rows of the matrix $\bD_{1:i}^{1/p}A_{1:i}$ picked by the algorithm when the rows of the matrix $\bD^{1/p} A$ are presented to it online in the row arrival model. The matrix $S_i \bD_{1:i}^{1/p}A_{1:i}$ has at most $O(T)$ rows. Note that the state of the  Algorithm~\ref{alg:l-infinity-coreset} does not change when it sees a row that has previously been seen. Thus, we can take $T$ to be an upper bound on the sum of online $\ell_2$ sensitivities of the matrix $\bD|_B^{1/p} B$ and by Theorem~\ref{thm:sum-of-online-sensitivities}, we obtain that $T = O(d\log n\log n\kappa^{\OL}(B))$ since $\bD$ scales the entries by at most a factor $n^{1/p}$. From here on, we use $\kappa^{\OL}$ to denote $\kappa^{\OL}(B)$.

Consider the $i$-th row and tag pair $(a_i, t_i) \in \R^{d} \times [N]$ being presented to the algorithm. First, we generate  $\bD_{ii} = \bg(t_i)$. Then we feed the row $\bD_{ii}^{1/p}a_i$ into the coreset construction algorithm. Define $\zeta_i$ as
\begin{align*}
	\zeta_i := \max_x \frac{|\la a_i, x\ra|^p}{\linf{S_i \bD_{1:i}^{1/p} A_{1:i} x}^p}.
\end{align*}
Note that we can compute $\zeta_i$ by solving the following convex optimization problem:
\begin{align*}
	\min_x&\, \linf{S_i \bD_{1:i}^{1/p}A_{1:i}x}\\
	\text{subject to}&\, \sum_{j=1}^d a_{ij}x_j = 1.
\end{align*}
If $\alpha$ is the optimal value of the above convex optimization problem, then $\zeta_i = (1/\alpha)^p$. We will now show bounds on $\zeta_i$ using the properties satisfied by the matrix $\bD$ and the coresets $S_i$. Let $i' \in [m]$ be such that the deduplicated version of matrix $A_{1:i}$ is $B_{1:i'}$. We have by construction of the matrix $\bD$ that for all $x$,
\begin{align*}
	\linf{\bD_{1:i}^{1/p}A_{1:i}x} = \linf{\bD^{1/p}|_{B_{1:i'}}B_{1:i'}x}
\end{align*}
which implies that
\begin{align*}
	\frac{\linf{\bD^{1/p}|_{B_{1:i'}}B_{1:i'}x}}{O(\sqrt{T})}\le \linf{S_i\bD^{1/p}_{1:i}A_{1:i}x} \le \linf{\bD^{1/p}|_{B_{1:i'}}B_{1:i'}x}.
\end{align*}
Thus, for any vector $x$,
\begin{align*}
	\frac{|\la a_i, x\ra|^p}{\linf{\bD^{1/p}|_{B_{1:i'}}B_{1:i'}x}^p}\le \frac{|\la a_i, x\ra|^p}{\linf{S_i \bD_{1:i}^{1/p}A_{1:i}x}^p} \le \frac{|\la a_i, x\ra|^p}{\linf{\bD^{1/p}|_{B_{1:i'}}B_{1:i'}x}^p}(CT)^{p/2}.
\end{align*}
Using Lemma~\ref{lma:upper-and-lower-bounds},
\begin{align*}
	&\frac{|\la a_i, x\ra|^p}{C^pd^{\max(3p/2+1, p/2+3)}\poly(\log \kappa^{\OL}, \log n)\lp{B_{1:i'}x}^p}\\
	&\le \frac{|\la a_i, x\ra|^p}{\linf{S_i \bD_{1:i}^{1/p}A_{1:i}x}^p}\\
	 &\le \frac{|\la a_i, x\ra|^p}{\lp{B_{1:i'}x}^p}(CT)^{p/2}C^pd^3\poly(\log \kappa^{\OL}, \log n).
\end{align*}
We thus have
\begin{align*}
	\frac{\tau^{\ell_p}_j(B)}{C^pd^{\max(3p/2+1, p/2+3)}\poly(\log \kappa^{\OL}, \log n)}\le \zeta_i
\end{align*}
and
\begin{align*}
     \zeta_i &\le (CT)^{p/2}C^pd^3\poly(\log n, \log \kappa^{\OL}) \cdot \tau^{\OL,\ell_p}_j(B)\\
				&\le C^{p/2}d^{p/2+3} \poly(\log n, \log \kappa^{\OL})\cdot \tau^{\OL,\ell_p}_j(B).
\end{align*}
Thus, $s_i := \zeta_i \cdot (C^pd^{\max(3p/2+1, p/2+3)}\poly(\log n, \log \kappa^{\OL}))$ is an upper bound on the \emph{offline} sensitivity of the row $b_j$ with respect to $B$. We also have $s_i \le d^{\max(2p+4,p+6)}\poly(\log\kappa^{\OL}, \log n)\tau_j^{\OL,\ell_p}(B)$. This upper bound helps us in bounding the number of rows sampled by the algorithm to construct a subspace embedding.

Thus, the algorithm which samples the last occurrence of a distinct row in the stream with probability based on $s_i$ will compute an $\ell_p$ subspace embedding for the deduplicated matrix $B$. The algorithm samples $d^{O(p)}\poly(\log n, \log \kappa^{\OL})\varepsilon^{-2}$ rows at the end, which follows from the upper bound on the probabilities with which each row in $B$ is sampled by the algorithm. By using a Chernoff bound, we can union bound over all $n$ items of the stream and conclude that the algorithm never needs more than $d^{O(p)}\poly(\log n, \log \kappa^{\OL})\varepsilon^{-2}$ space. To store the random hash function $\bh$, the algorithm uses only $\poly(d, \log N, \log\log \kappa^{\OL})$ bits as the hash family used is required to be $O(d\log(n) + \poly(\log\log \kappa^{\OL}, \log n))$-wise independent.
\end{proof}
\section{Analysis of Alternate Algorithm in Section~\ref{sec:alternate}}
As usual, assume that $A \in \R^{n \times d}$ denotes the matrix formed by all the rows in the stream and let $\dedup(A)$ denote the matrix formed by the rows corresponding to distinct tags. 

Fix a vector $x$ with $\lp{\dedup(A)x} = 1$. For $i,j \in [n]$, we define the matrix $A^{(j)}_i$ as follows:
\begin{itemize}
    \item If $i \le j$, the matrix $A^{(j)}_i$ is formed by the rows of $\dedup(A_{1:i})$ that do not appear again until end of time $j$. Notably, $A^{(j)}_j = \dedup(A_{1:j})$.
    \item If $i > j$, the matrix $A^{(j)}_i$ is defined to be $\dedup(A_{1:j})$.
\end{itemize}

Let $M_i$ be the matrix formed after the end of processing $i$ elements in the stream by Algorithm~\ref{alg:alternate-algorithm}. Note that the matrix $M_i$ is \emph{random}. For $j \in [n]$, we define $M_i^{(j)}$ as follows:
\begin{itemize}
    \item If $i \le j$, the matrix $M_i^{(j)}$ is formed by the rows of $M_i$ that will not be deleted by the end of $j$-th iteration of the algorithm i.e., only those rows of $M_i$ with the tags that do not reappear before the end of processing $j$-th stream element. We also have $M_j^{(j)} = M_j$.
    \item If $i > j$, the matrix $M_i^{(j)}$ is defined to be $M_j$.
\end{itemize}
We define $n$ martingales $X^{(1)} = (X_0^{(1)}, X_1^{(1)} \ldots, ), \ldots, X^{(n)} = (X_0^{(n)}, X_1^{(n)}, \ldots)$ based on the execution of Algorithm~\ref{alg:alternate-algorithm}. Set $X^{(j)}_0 = 0$ for all $j$. We now define $X^{(j)}_i$ based on the values $X^{(1)}_{i-1}, \ldots, X^{(n)}_{i-1}$, the probability $p_i$ in the $i$-th iteration of the Algorithm~\ref{alg:alternate-algorithm} and the random choice of sampling the $i$-th row by the algorithm.

If $|X_{i-1}^{(j)}| > \varepsilon$ for any $j$, then set $X_i^{(j)} = X_{i-1}^{(j)}$ for all $j$. Otherwise, for $j < i$, set $X^{(j)}_i = X^{(j)}_{i-1}$. For $j \ge i$, if the tag $t_i$ does not appear again before the end of time $j$, then set $X_i^{(j)} := X_{i-1}^{(j)} + (1/p_i - 1)|\la a_i, x\ra|^p$ if the algorithm samples row $a_i$ otherwise set $X_i^{(j)} := X_{i-1}^{(j)} - |\la a_i, x\ra|^p$. If the tag $t_i$ appears again before the end of time $j$, set $X^{(j)}_i = X^{(j)}_{i-1}$. 

Assuming that the absolute values of \emph{all} the random variables $X_i^{(j)}$ do not exceed $\varepsilon$, we have
\begin{align*}
    X_i^{(j)} = \|M_i^{(j)}x\|_p^p - \|A_i^{(j)}x\|_p^p.
\end{align*}
We now use Freedman's inequality to show that with a large probability for all $i, j \in [n]$, we have $|X_i^{(j)}| \le \varepsilon$.

The only interesting case is when the value of $X_i^{(j)}$ is different from $X_{i-1}^{(j)}$. Hence the probability $p_i = \alpha \tau_i < 1$ and $|X^{(j)}_{i-1}| \le \varepsilon$ for all $j$ and especially $|X^{(i-1)}_{i-1}| \le \varepsilon$. Now,
\begin{align*}
    \tau_i = \max_y \frac{|\la a_i,y\ra|^p}{\lp{M_{i-1}y}^p} \ge \frac{|\la a_i, x\ra|^p}{\lp{M_{i-1}x}^p}.
\end{align*}
Hence $1/\tau_i \le \lp{M_{i-1}x}^p/|\la a_i, x\ra|^p \le (1 + \varepsilon)/|\la a_i, x\ra|^p$ since $\lp{M_{i-1}x}^p \le \lp{A_{i-1}^{(i-1)}x}^p + \varepsilon \le \lp{\dedup(A)x}^p + \varepsilon \le 1 + \varepsilon$ and therefore $1/\tau_i \le 2/|\la a_i, x\ra|^p$. Now,
\begin{align*}
    |X_i^{(j)} - X_{i-1}^{(j)}| \le \frac{1}{p_i}|\la a_i, x\ra|^p \le \frac{2}{\alpha}
\end{align*}
and
\begin{align*}
    \E[(X_i^{(j)} - X_{i-1}^{(j)})^2] \le \frac{1}{p_i}|\la a_i, x\ra|^{2p} = \frac{1}{\alpha \tau_i}|\la a_i, x\ra|^{2p} \le \frac{2}{\alpha}|\la a_i, x\ra|^p.
\end{align*}
As for each martingale $X^{(j)}$, a row and tag pair $(a_i, t_i)$ is considered only once, the predictable quadratic variation of the martingale $X^{(j)}$ defined as $\sum_i \E[(X_i^{(j)} - X_{i-1}^{(j)})^2]$ satisfies
\begin{align*}
   \sum_i \E[(X_i^{(j)} - X_{i-1}^{(j)})^2] \le (2/\alpha)\sum_{a_i \in \dedup(A_{1:j})}|\la a_i, x\ra|^p \le (2/\alpha)
\end{align*}
 Now, we can apply Freedman's inequality and conclude that if $\alpha = O(d\log n/\varepsilon^2)$, then with probability $\ge 1 - \exp(-O(d\log n))$, for all the martingales $X^{(j)}$ and all $i$, $|X^{(j)}_i| \le \varepsilon$ simultaneously by a union bound over $n$ martingales. Hence,
\begin{align*}
    |X_n^{(n)}| = |\lp{M_n^{(n)}x}^p - \lp{A_n^{(n)}x}^p| \le \varepsilon
\end{align*}
and
\begin{align*}
    \lp{M_nx}^p = (1 \pm \varepsilon)\lp{\dedup(A)x}^p.
\end{align*}
We can then apply union bound over a net and conclude that $M$ at the end of the algorithm is a subspace embedding with probability $\ge 1 - 1/\poly(n)$. By a union bound over each point in the stream, we obtain that we have a subspace embedding at each point of the stream. This then gives an upper bound on $\tau_i$s that are computed in the stream and then we obtain that space required by the streaming algorithm is bounded.
\section{Missing Proofs from Section~\ref{sec:lower-bounds}}
\begin{proof}[Proof of Theorem~\ref{thm:lower-bound-deterministic-algorithms}]
First we define the Equal-vs-Spread problem that we use to prove our lower bound.
\begin{definition}[Equal-vs-Spread]
    In the $(n,t)$ Equal-vs-Spread problem, there are $t$ players and player $i$ receives $x_i \subseteq [n]$ of size $|x_i| = \ceil{\beta n}$. The task is to distinguish between the following cases:
    \begin{enumerate}
        \item $x_1 = x_2 = \ldots = x_n$
        \item $|x_1 \cup x_2 \cup \ldots \cup x_n| \ge \gamma n$
    \end{enumerate}
\end{definition}
We denote the problem using the notation $\textnormal{EQ-SPRD}^{\beta,\gamma}_{n,t}$. Now we state the lower bound from \cite{chakrabarti2016strong} on the communication complexity of ``discreet protocols'' solving this problem.
\begin{theorem}[{{\cite[Theorem~3.4]{chakrabarti2016strong}}}]
    For all values of $t \ge 2$, $\beta > 0$, $\gamma = \beta t(1-e\beta t) > \beta$ and sufficiently large integral $n$, we have $\textnormal{DD}(\textnormal{EQ-SPRD}^{\beta,\gamma}_{n,t}) \ge 2e\beta^2 n - 2\log t - \Theta(1)$.
\end{theorem}
Here $\text{DD}(\cdot)$ denotes the minimum, over all the protocols that solve the problem, of the maximum communication of any player.

Suppose there is a space $s$ streaming algorithm that for any matrix $A$, computes an $\ell_p$ subspace embedding $B'$ satisfying for all vectors $x$,
\begin{align*}
    \lp{\dedup(A)x} \le \lp{B'x} \le C\lp{\dedup(A)x}.
\end{align*}
Now consider the following way of using the streaming algorithm to solve the $\textnormal{EQ-SPRD}^{\beta,\gamma}_{n,t}$ problem. First, player $1$ depending on the subset $x_1 = \set{i_1,\ldots,i_{\beta n}}$ they possess creates the stream of pairs $(1, i_1), (1, i_2), \ldots, (1, i_{\beta n})$ and feeds it to the streaming algorithm. Here note that $i_1,\ldots,i_{\beta n}$ are passed on as tags to the streaming algorithm. Then player $1$ communicates the state of the streaming algorithm using $s$ bits of communication to player $2$ who then creates a stream depending on the subset they possess and feeds the stream to the streaming algorithm and passes the state of the algorithm to player $3$ and so on. If $A$ denotes the $t\beta n \times 1$ matrix formed by the stream, then $\dedup(A)$ has $|x_1 \cup \ldots \cup x_t|$ number of rows all equal to $1$.

If at the end of the stream, player $t$ computes an $\ell_p$ subspace embedding $B'$ of distortion $C$ for $\dedup(A)$, then
\begin{align*}
    |x_1 \cup \ldots \cup x_t|^{1/p} \le \lp{B' \cdot 1} \le C|x_1 \cup \cdots \cup x_t|^{1/p}.
\end{align*}
If $C \le (\gamma/\beta)^{1/p}$, then player $t$ can determine if all the players received the same sets or if the union of sets they received has a size $\ge \gamma n$. Note that in this protocol, the total communication by any player is at most $2s$ and therefore any deterministic streaming algorithm that computes an $\ell_p$ subspace embedding of distortion $(\gamma/\beta)^{1/p}$ for a deduplicated matrix must use $s \ge (2e\beta^2 n - 2\log t - \Theta(1))/2$ space. Setting $t = 1/(2e\beta)$, $\gamma = 1/4e$, we obtain using the above theorem that any $(1/4e\beta)^{1/p}$ distortion streaming algorithm for constructing an $\ell_p$ subspace embedding for the deduplicated matrix formed from a matrix of $n/2e$ rows must use $s \ge (2e\beta^2n -2 \log t - \Theta(1))/2$ space. By setting $C = (1/4e\beta)^{1/p}$, we obtain that any deterministic streaming algorithm with distortion $C$ must use
\begin{align*}
    \Omega\left(\frac{n}{C^{2p}} - p \log(C)\right)
\end{align*}
bits of space in contrast to the algorithms for non-deduplicated matrices.
\end{proof}
\begin{proof}[Proof of Theorem~\ref{thm:lower-bounds-sketching-algorithms}]
Suppose that the sketching matrix $\bS$ has $s$ rows. We prove the theorem by reducing from the multi-party set-disjointness problem. Consider the $n \times d$ matrix $A$ whose columns are given by the indicator vectors of the sets possessed by each of the $d$ players. If all the sets are mutually disjoint, then all of the rows of $\dedup(A)$ are either coordinate vectors or a zero vector. If there is a single element common among all the sets, then $\dedup(A)$ consists of a row of all ones. Consider $x = 1_d$. Thus, when all the sets are mutually disjoint, $\lp{\dedup(A)x} \le d^{1/p}$ and if all the sets intersect in one item, $\lp{\dedup(A)x} \ge d$. Thus, an $\ell_p$ subspace embedding with distortion at most $d^{1/2-1/2p}$ can differentiate between the two cases of the $d$ player set disjointness problem.

If all the players sample the random matrix $\bS$ using shared randomness and write out the product $\bS x_i$ where $x_i$ is the indicator vector of the set the $i$-th player has, then the total communication is given by $\tilde{O}(sd)$ bits (assuming that the entries of $\bS$ have $O(\log n)$ bits) where $s$ is the size of the sketch. But using the lower bound of $\Omega(n/d)$ on the communication of any protocol that solves the set disjointness problem, we obtain that $s = \tilde{\Omega}(n/d^2)$. Hence, any random sketching matrix $\bS$ that can be used to compute an $\ell_p$ subspace embedding with distortion $C = d^{1/2-1/2p}$  for the deduplicated matrix must have $\tilde{\Omega}(n/d^2)$ rows.
\end{proof}
\section{Missing Details from Section~\ref{sec:turnstile}}
\begin{theorem}
    Given a matrix $A \in \R^{n \times d}$, $p \in [1,\infty)$, accuracy parameter $\varepsilon$ and $s \ge d^{O(p)}\poly(\log n)$, the Algorithm~\ref{alg:alternate-algorithm} returns a matrix $M$ with $d^{O(p)}\poly(\log n)/\varepsilon^2$ rows such that with probability $\ge 1 - 1/\poly(\log n)$, the matrix $M$ satisfies for all $x$,
    \begin{align*}
        \lp{Mx}^p = (1 \pm \varepsilon)\lp{Ax}^p.
    \end{align*}
    \label{thm:offline-recursive-lp}
\end{theorem}
\begin{proof}
Consider an arbitrary matrix $A$ with $n$ rows. For $i \in [n]$, recall that $\tau_i^{\ell_p}(A)$ is the $\ell_p$ sensitivity of the $i$-th row with respect to the matrix $A$. We will always index the rows with their index in $A$ i.e., for $i \in \bS$, we say that the $i$-th row of $A_{\bS}$ is $a_i$.

Let $\bS \subseteq [n]$ be a random subset obtained by independently sampling each $i \in [n]$ to be in $\bS$ with probability $1/2$. For $i \in [n]$, define as in the algorithm,
\begin{align*}
    \tau_i^{\bS} = \min\left(1,\max_{x} \frac{|\la a_i, x\ra|^p}{\lp{A_{\bS}x}^p}\right).
\end{align*}
Clearly, $\tau_i^{\bS} \ge \tau_i^{\ell_p}(A)$ as $\lp{A_{\bS}x}^p \le \lp{Ax}^p$ for all $x$ with probability $1$ over $\bS$. We shall now bound $\sum_{i \in [n]}\tau_i^{\bS} = \sum_{i \in \bS}\tau_i^{\bS} + \sum_{i \notin \bS}\tau_i^{\bS}$. We first note that for $i \in \bS$, $\tau_i^{\bS} = \tau_{i}^{\ell_p}(A_{\bS})$. Hence, $\sum_{i \in \bS}\tau_i^{\bS} \le d^{\max(p/2,1)}$. Now, we bound $\sum_{i \notin \bS}\tau_i^{\bS}$. For $i \notin \bS$, clearly we have
\begin{align*}
    \tau_i^{\bS} \le 2\tau_{i}^{\ell_p}(A_{\bS \cup i}).
\end{align*}
Hence, $\sum_{i \notin \bS}\tau_i^{\bS} \le 2\sum_{i \notin \bS}\tau_i^{\ell_p}(A_{\bS \cup i})$. Now, we bound $\sum_{i \notin \bS} \tau_i^{\ell_p}(A_{\bS \cup i})$ with a high probability. 
\begin{align*}
    \E_{\bS}[\sum_{i \notin \bS}\tau_i^{\ell_p}(A_{\bS \cup i}) \mid |\bS| = t] &= \sum_{S \subseteq [n], |S| = t}\Pr[\bS  = S \mid |\bS| = t]\sum_{i \notin S}\tau_i^{\ell_p}(A_{S \cup i})\\
    &=\sum_{T \subseteq [n], |T| = t+1}\sum_{i \in T}\Pr[\bS = T \setminus i \mid |\bS| = t]\tau_i^{\ell_p}(A_T).
\end{align*}
As $\Pr[\bS = T \setminus i \mid |\bS| = t]$ is independent of $i$, we obtain that
\begin{align*}
    \E_{\bS}[\sum_{i \notin \bS}\tau_i^{\ell_p}(A_{\bS \cup i}) \mid |\bS| = t] &=\sum_{T \subseteq [n], |T| = t+1}\sum_{i \in T}\Pr[\bS = T \setminus i \mid |\bS| = t]\tau_i^{\ell_p}(A_T)\\
    &= \sum_{T \subseteq [n], |T| = t+1} \frac{\sum_{i \in T}\Pr[\bS = T \setminus i \mid |\bS| = t]}{t+1} \sum_{i \in T}\tau_i^{\ell_p}(A_T)].
\end{align*}
Using $\sum_{i \in T}\tau_i^{\ell_p}(A_T) \le d^{\max(p/2,1)}$, we get
\begin{align*}
    \E_{\bS}[\sum_{i \notin \bS} \tau_i^{\ell_p}(A_{\bS \cup i}) \mid |\bS| = t] \le \frac{d^{\max(p/2,1)}}{t+1}\sum_{T \subseteq [n], |T|=t+1}\sum_{i \in T}\Pr[\bS = T \setminus i \mid |\bS| = t] \le \frac{n}{t+1}d^{\max(p/2,1)}.
\end{align*}
By an application of the Chernoff bound, we have with high probability that $|\bS| \ge n/4$. Conditioned on the event that $|\bS| \ge n/4$, the above expectation property implies that $\sum_{i \notin \bS}\tau_i^{\ell_p}(A_{\bS \cup i}) \le O(d^{\max(p/2,1)}\log n)$ with probability $\ge 1 - 1/(C'\log n)$ for a large enough constant $C'$ by Markov inequality. Overall, we have that with probability $\ge 1 - 1/C\log n$, 
\begin{align*}
    \sum_{i \in [n]}\tau_i^{\bS} \le O(d^{\max(p/2,1)}\log n).
\end{align*}
Now condition on the matrix $M_{\bS}$ being an $\ell_p$ subspace embedding for $A_{\bS}$ (by induction). We then have
\begin{align*}
    (1/2)\tau_i^{\bS} \le \tau_i^{M_\bS} \le 2\tau_i^{\bS}
\end{align*}
by the subspace embedding property. Thus, with large probability, for all $i \in [n]$, 
\begin{align*}
    \frac{\tau_i^{M_\bS}}{\sum_i \tau_i^{M_\bS}} \ge \frac{\tau_i^{\ell_p}(A)}{C'' d^{\max(p/2,1)}\log n} \ge \frac{\tau_i^{\ell_p}(A)}{\sum_i \tau_i^{\ell_p}(A)}\frac{\sum_i \tau_i^{\ell_p}(A)}{C''d^{\max(p/2,1)}\log n} \ge \frac{\tau_i^{\ell_p}(A)}{\sum_{i}\tau_i^{\ell_p}(A)} \frac{1}{C''d^{\max(p-1,2)}\log n}
\end{align*}
where we used the lower bound on the sum of $\ell_p$ sensitivities of a rank $d$ matrix. 

Thus, sampling from a distribution proportional to $\tau_i^{M_\bS}$, with a large probability, corresponds to sampling from an approximate $\ell_p$ sensitivity distribution and hence the algorithm returns an $\varepsilon$ subspace embedding for $A$ with a large probability.
\end{proof}
\subsection{The Algorithm}
Let $\enc(a) \in [N]$ denote the encoding of a row $a$ as a nonnegative integer and for $i \in [N]$, let $\dec(i)$ denote the row $a \in \set{-M, \ldots, M}^d$ for which $\enc(a) = i$. Here onwards, we use $a$ and $\enc(a)$ interchangeably. Hence the stream of updates can also equivalently be seen as updating an $N$ dimensional vector ``$v$''. As seen above, using the $L_0$ estimator, we can estimate the number of non-zero coordinates in the vector $v$ at the end of the stream and using the $L_0$ sampler we can sample an approximately uniformly random nonzero coordinate in the vector $v$, which is equivalent to sampling a uniformly random row in the matrix $\dedup(A)$.

Let $t$ be the number of passes of the algorithm for a parameter $t$ to be defined later. Let $\bh_1,\ldots,\bh_t : [N] \rightarrow \set{0,1}$ be $t$ independent fully random hash functions. We will remove this assumption later by using Nisan's pseudorandom generator.

Define random subsets $\bS_1, \bS_2,  \ldots, \bS_t \subseteq [N]$ as follows: an index $i \in \bS_j$ iff \[\bh_j(i) = \bh_{j+1}(i) = \cdots = \bh_t(i) = 1.\] 
It is clear that the subsets $\bS_1,\ldots,\bS_t$ satisfy $\bS_1 \subseteq \bS_2 \subseteq \cdots \subseteq \bS_t$. Let $\Encs$ denote the set $\set{\enc(b_1), \ldots, \enc(b_r)}$. We also define $\bS_{t+1}$ to be the set $[N]$. Let $b_1$, $b_2$, \ldots, $b_r$ be the rows of the matrix $\dedup(A)$. To implement the recursive $\ell_p$ sensitivity sampling algorithm (Algorithm~\ref{alg:recursive-sampling-algorithm}) on the matrix $\dedup(A)$, we need to sub-sample rows of the matrix $\dedup(A)$ recursively. The sets $\bS_1 \cap \Encs, \bS_2 \cap \Encs, \ldots, \bS_t \cap \Encs$ serve as the recursively sub-sampled sets of rows in the algorithm. We further define $\dedup(A)_{\bS_i}$ to be the matrix formed by the rows in $\bS_i \cap \Encs$ and we let 
\begin{align*}
    \tau_i^{\bS_j} := \min\left(1, \max_x\frac{|\la \dec(i), x\ra|^p}{\lp{\dedup(A)_{\bS_j} \cdot x}^p}\right).
\end{align*}
We condition on the following event: for all $i=1,\ldots,t$
\begin{align*}
    \sum_{i \in \bS_{j+1} \cap \Encs} \tau_i^{\bS_j} \le O(d^{\max(p/2,1)}\log n).
\end{align*}
For $t = O(\log n)$, proof of Theorem~\ref{thm:offline-recursive-lp} shows that this event holds with probability $\ge 99/100$.

We set $t$ such that the set $\bS_1 \cap \Encs$ has  $\le \poly(d)$ rows. The algorithm makes a pass over the stream of rows and cares only about updates to those $a_i$s with $\bh_1(a_i) = \cdots \bh_t(a_i) = 1$. Let $v_1$ be the $\poly(n)^d$ dimensional vector tracking the updates to those rows $a$ with $\bh_1(a) = \cdots = \bh_t(a) = 1$. Conditioned on $|\bS_1| \le \poly(d)$, the vector $v_1$ has at most $\poly(d)$ nonzero entries at the end of processing the stream. Hence, the vector $v_1$ can be extracted using a $\poly(d)$-sparse recovery data structure using $O(\poly(d)\log n)$ bits of space. Using the recovered vector $v_1$, the matrix $\dedup(A)_{\bS_1}$ can be reconstructed. Let $M_1$ be a $1/2$ $\ell_p$ subspace embedding for the matrix $\dedup(A)_{\bS_1}$ and assume that the matrix $M_1$ has $O(\poly(d)\log n)$ rows. (Setting $M_1 := \dedup(A)_{\bS_1}$ itself satisfies the guarantees; we describe it this way to be consistent with the rest of the rounds).

Assume that we have constructed a $1/2$ $\ell_p$ subspace embedding $M_j$ for the matrix $\dedup(A)_{\bS_j}$. We will now argue how to construct a $1/2$ $\ell_p$ subspace embedding for the matrix $\dedup(A)_{\bS_{j+1}}$. The algorithm makes a pass over the rows and for each row $a$ in the stream satisfying $\bh_{j+1}(a) = \cdots = \bh_{t}(a) = 1$, computes the sensitivity approximation 
\begin{align*}
    \tau^{M_j}(a) = \min\left(1, \max_x \frac{|\la a, x\ra|^p}{\lp{M_j x}^p}\right).
\end{align*}
Note that if $M_j$ is a subspace embedding for $\dedup(A)_{\bS_j}$, then $\tau^{M_j}(a)$ is a constant fraction approximation for $\tau^{\bS_j}(a)$ for all $a$.

The algorithm discards all the rows $a$ in the stream that do not satisfy $\bh_{j+1}(a)  = \cdots = \bh_t(a) = 1$. We now partition the rows $a$ into $b$ \emph{buckets} $P_1, \ldots, P_b$ such that $a \in P_{\ell}$ iff
\begin{align*}
    \frac{1}{2^{\ell}} \le \tau^{M_j}(a) \le \frac{1}{2^{\ell-1}}.
\end{align*}
We pick $b = O(\log n)$ such that every non-zero row $a \in \set{-M, \ldots, M}^d$ falls into one of the buckets. For each bucket $\ell \in [b]$, we maintain an $N$ dimensional vector $v^{(\ell)}_{j+1}$ so that the vector $v^{(\ell)}_{j+1}$ tracks the updates to those rows $a$ in the stream with $1/2^{\ell} \le \tau^{M_j}(a) \le 1/2^{\ell-1}$. $L_0$ sampling of the vector $v_{j+1}^{(\ell)}$ then corresponds to sampling a uniform random row among the rows in $\bS_{j+1} \cap \Encs$ that gets hashed into bucket $\ell$. Let $\Est_1,\ldots,\Est_b$ denote the estimates such that
\begin{align*}
    (9/10)\lzero{v^{(\ell)}_{j+1}} \le \Est_{\ell} \le (11/10)\lzero{v^{(\ell)}_{j+1}}
\end{align*}
which can be obtained by the $L_0$ estimation algorithm described earlier.
At the end of the stream, sample a random bucket $\bell \in [b]$ such that \[\Pr[\bell = i] = \frac{\Est_{i} \cdot 2^{-i}}{\sum_{i \in [b]} \Est_{i} \cdot 2^{-i}}.\] Then use an approximate $L_0$ sampler to sample a non-zero coordinate of the vector $v^{(\bell)}_{j+1}$ to obtain an index $\br \in [\poly(n)^d]$ which corresponds to a row $\enc(\br)$.  Now consider an arbitrary row $b_i \in \bS_{j+1} \cap \Encs$. Let $\ell_i \in [b]$ be such that $b_i \in P_{\ell_i}$. Finally, we have, conditioned on non-failure of the $L_0$ sampler that,
\begin{align*}
    \frac{2^{-\ell_i}\Est_{\ell_i}}{\sum_{\ell \in [b]} 2^{-\ell}\Est_{\ell}} \left[\frac{11}{10\Est_{\ell_i}}\right] \pm O(1/\poly(n)) \ge \Pr[\enc(\br) = b_i]
\end{align*}
and
\begin{align*}
    \Pr[\enc(\br) = b_i] \ge \frac{2^{-\ell_i}\Est_{\ell_i}}{\sum_{\ell \in [b]} 2^{-\ell}\Est_{\ell}} \left[\frac{9}{10\Est_{\ell_i}}\right] \pm O(1/\poly(n)).
\end{align*}
We then obtain
\begin{align*}
    \Pr[\enc(\br) = b_i] &\ge \frac{\tau^{\bS_j}(a_i)}{C\sum_{i \in \bS_{j+1} \cap \Encs} \tau^{\bS_j}(a_i)}\\
    &\ge \frac{\tau^{\bS_{j+1}}(a_i)}{d^{O(p)}\log n\sum_{i \in \bS_{j+1} \cap \Encs}\tau^{\bS_{j+1}}(a_i)}.
\end{align*}
Hence, sampling $O(d^{O(p)}\poly(\log n))$ rows from the above distribution gives a $1/2$ $\ell_p$ subspace embedding for the matrix $\dedup(A)_{\bS_{j+1}}$. 

In the final round, we instead sample $O(d^{O(p)}\poly(\log n)/\varepsilon^2)$ rows to obtain an $\varepsilon$ subspace embedding for the matrix $\dedup(A)$. Overall, we use at most $O(d^{O(p)}\poly(\log n)/\varepsilon^2)$ $L_0$ samplers in each round and hence using a space of $O(d^{O(p)}\poly(\log n)/\varepsilon^2)$ bits for the whole algorithm, we can condition on the non-failure of all the $L_0$ samplers, $L_0$ estimators in the streaming algorithm which proves the correctness.

\section{Missing Proofs from Section~\ref{sec:bounded-entries}}
\begin{lemma}
Let $a_1,\ldots,a_m$ be $m$ positive integers satisfying $1 \le a_i \le \poly(d)$. Let $\bX$ be a random variable such that
\begin{align*}
    \Pr[\bX = a_i] = (1/m)
\end{align*}
for all $i$. Let $\bX_1,\ldots,\bX_t$ be independent copies of the random variable $\bX$. Then if $t \ge C\varepsilon^{-2}\poly(d)^2\log(1/\delta)$ for a large enough constant $C$,
\begin{align*}
    \Pr\left[\left|\frac{m(\bX_1 + \ldots + \bX_t)}{t} - \sum_{i=1}^m a_i\right| \ge \varepsilon\sum_{i=1}^m a_i\right] \le \delta
\end{align*}
\label{lma:hoeffding-application}
\end{lemma}
\begin{proof}
    Note that $\E[\bX] = (1/m)\sum_{i=1}^m a_i$ and $|\bX| \le \poly(d)$ with probability $1$. By applying Hoeffding's inequality,
    \begin{align*}
        \Pr\left[\left|\sum_{i=1}^t \bX_i - (t/m)\sum_{i=1}^m a_i\right| \ge \alpha\right] \le 2\exp\left(-\frac{2\alpha^2}{t(\poly(d))^2}\right).
    \end{align*}
    Setting $\alpha = \varepsilon (t/m) \sum_{i=1}^m a_i$, we obtain
    \begin{align*}
        \Pr\left[\left|\sum_{i=1}^t \bX_i - (t/m)\sum_{i=1}^m a_i\right| \ge \varepsilon(t/m)\sum_{i=1}^m a_i\right] \le 2\exp\left(-\frac{2\varepsilon^2(t/m)^2(\sum_{i=1}^m a_i)^2}{t(\poly(d))^2}\right).
    \end{align*}
    As $a_i \ge 1$ for all $i$, we have $(1/m)\sum_{i=1}^m a_i \ge 1$ and therefore
    \begin{align*}
    \Pr\left[\left|\sum_{i=1}^t \bX_i - (t/m)\sum_{i=1}^m a_i\right| \ge \varepsilon(t/m)\sum_{i=1}^m a_i\right] \le 2\exp\left(-\frac{2\varepsilon^2t}{(\poly(d))^2}\right).
    \end{align*}
    By picking $t = \Theta(\varepsilon^{-2}\poly(d)^2\log(1/\delta))$ we obtain the result.
\end{proof}
\section{Analysis of Adversarial Robust algorithm in Section~\ref{sec:adversarial}}
\subsection{The Setting}
The algorithm sees pairs of rows and tags $(a_1,t_1), \ldots,(a_n, t_n) \in \R^d \times [N]$ in the stream generated by an adaptive adversary with the guarantee that $\kappa^{\OL}(\dedup(A)) \le \kappa^{\OL}$. After each $i \in [n]$, the algorithm has to output an $\ell_p$ sensitivity estimate $\zeta_i$ of row $a_i$ with respect to the matrix $\dedup(A_{1:i})$. We want the algorithm to satisfy the following guarantee: with probability $\ge 9/10$, for all $i \in [n]$
\begin{align*}
    \zeta_i \approx \max_x \frac{|\la a_i, x\ra|^p}{\lp{\dedup(A_{1:i})x}^p}.
\end{align*}
By Yao's lemma, we can assume that the adversary is deterministic and generates $(a_{i+1}, t_{i+1})$ as a function of the outputs $\zeta_1, \ldots, \zeta_i$ of the algorithm.
\subsection{The Algorithm}
For a parameter $\ell$ to be decided later, let $\bD^{(1)}, \ldots, \bD^{(\ell)}$ be independent matrices formed by independent hash functions $\bg^{(j)}$ so that $\bD^{(j)}_{ii} = \bg^{(j)}(t_i)$ for $j \in [\ell]$. Here $\bg^{(j)}$ is a hash function as defined in \eqref{eqn:definition-of-g}. 

If a matrix $A \in \R^{n \times d}$ is constructed independent of the randomness of an embedding matrix $\bD^{(j)}$, then by Lemma~\ref{lma:upper-and-lower-bounds}, with probability $\ge 1 - \delta$, for all $i \in [n]$ and for all $x \in \R^d$,
\begin{align*}
    \linf{((\bD^{(j)})^{1/p}A)_{1:i}x} \approx_{} \lp{\dedup(A_{1:i})x}.
\end{align*}
Here the approximation factor is $d^{O(1)}\poly(\log n, \log \kappa^{\OL}, \log(1/\delta))/\delta^{1/p}$. 
We also have that the sum of online $\ell_2$ leverage scores of the matrices $\dedup((\bD^{(1)})^{1/p}A)$, $\ldots$, $\dedup((\bD^{(\ell)})^{1/p}A)$ is bounded by $T = O(d \poly(\log n, \log \kappa^{\OL}))$. Let $S^{(j)}_i$ be the coreset constructed for $((\bD^{(j)})^{1/p}A)_{1:i}$ by the deterministic coreset construction algorithm of \cite{woodruff2022high} which gives for all $j$ and $i$ that
\begin{align*}
    \linf{\bS_i^{(j)}((\bD^{(j)})^{1/p}A)_{1:i}x} \approx \linf{((\bD^{(j)})^{1/p}A)_{1:i} x}.
\end{align*}
The approximation factor in the above inequality is $O(\sqrt{T})$.

We will now describe the sketch-switching procedure. Assume that the algorithm has seen the updates $(a_1,t_1), \ldots (a_i, t_i)$ in the stream and currently using the matrix $\bD^{(j)}$ to compute approximate sensitivities as in Algorithm~\ref{alg:one-pass-arbitrary-order}. As $\bD^{(j)}$ is used in computing estimates of the sensitivities, the information about $\bD^{(j)}$ leaks to the adversary and the adversary may be able to create updates that break the embedding. So, we use another \emph{currently} hidden embedding matrix $\bD^{(j+1)}$ to decide when the embedding $\bD^{(j)}$ becomes stale. Concretely, let $i_{\text{start}} \in [n]$ be the index when the algorithm starts to use $\bD^{(j)}$ to estimate sensitivities. For $i \ge i_{\text{start}}$, the sensitivity estimate is computed as
\begin{align*}
    \zeta_i := \max_x \frac{|\la a_i, x\ra|^p}{\linf{S^{(j)}_{i_{\text{start}}} ((\bD^{(j)})^{1/p}A)_{1:i_{\text{start}}}x}^p}.
\end{align*}
As adversary is oblivious to the randomness of $\bD^{(j)}$ while creating the updates $(a_1,t_1), \ldots, (a_{i_{\text{start}}}, t_{i_{\text{start}}})$ we have that with probability $\ge 1 - \delta$, for all $x$,
\begin{align*}
    \linf{S^{(j)}_{i_{\text{start}}} ((\bD^{(j)})^{1/p}A)_{1:i_{\text{start}}}x} \approx \lp{\dedup(A_{1:i_{\text{start}}})x}.
\end{align*}
Hence, $d^{O(p)}(\poly(\log n, \log \kappa^{\OL})/\delta) \zeta_i$ is an upper bound on the sensitivity of the $i$-th row with respect to the matrix $\dedup(A_{1:i})$. We now want to show that $\zeta_i$ can not be too large as compared to the online sensitivity of the $i$-th row. 

In the adversarially robust algorithm, we use another embedding $\bD^{(j+1)}$ to compute when the embedding $((\bD^{(j)})^{1/p}A)_{1:i_{\text{start}}}$ becomes stale. Formally after seeing a row $i$, for a parameter $L$, we switch from $\bD^{(j)}$ to $\bD^{(j+1)}$ if there exists a vector $\tilde{x}$ such that
\begin{align*}
    \linf{S^{(j+1)}_i ((\bD^{(j+1)})^{1/p}A)_{1:i}\tilde{x}} > L \linf{S_{i_{\text{start}}}^{(j)} ((\bD^{(j)})^{1/p}A)_{1:i_{\text{start}}}\tilde{x}}.
\end{align*}
As rows of $A$ do not depend on the randomness until the switch happens, we have that with probability $\ge 1 - \delta$, for all $i$ until the switch and for all $x$,
\begin{align*}
    \lp{\dedup(A)_{1:i}x} \approx \linf{S_{i}^{(j+1)} ((\bD^{(j+1)})^{1/p}A)_{1:i}x}.
\end{align*}
If switch happens after row $i$, we then have that there is a vector $\tilde{x}$ that satisfies
\begin{align*}
    \lp{\dedup(A)_{1:i}\tilde{x}} > \frac{L\delta^{1/p}}{\poly(d,\log n, \log \kappa^{\OL})}\lp{\dedup(A)_{1:i_{\text{start}}}\tilde{x}}. 
\end{align*}
Let $L$ be large enough $\poly(d, \log n, \log \kappa^{\OL})/\delta^{1/p}$ such that we have
\begin{align*}
    \lp{\dedup(A)_{1:i}\tilde{x}} > 4\lp{\dedup(A)_{1:i_{\text{start}}}\tilde{x}}.
\end{align*}
Let $P$ be the set of indices for the matrix $\dedup(A)$ as in Theorem~\ref{thm:partition-theorem}. The above condition implies that there exists an index $i_{\text{mid}} \in P$ satisfying $i_{\text{start}} < i_{\text{mid}} \le i$. As $|P| = d^{O(p)}\poly(\log n, \log \kappa^{\OL})$, we obtain that the switch happens at most $d^{O(p)}\poly(\log n, \log \kappa^{\OL})$ number of times. The switching ensures that for all $i$, 
\begin{align*}
    \zeta_i = \max_x\frac{|\la a_i, x\ra|^p}{\linf{S_{i_{\text{start}}} ((\bD^{(j)})^{1/p}A)_{1:i_{\text{start}}}x}^p} \le L^p d^{O(p)}(\poly(\log n, \log \kappa^{\OL})/\delta) \max_x \frac{|\la a_i, x\ra|^p}{\lp{\dedup(A_{1:i})x}^p}.
\end{align*}
By setting $\delta = 1/(d^{O(p)}\poly(\log n, \log \kappa^{\OL}))$, we obtain that
\begin{align*}
    \zeta_i \le d^{O(p)}\poly(\log n, \log \kappa^{\OL})\tau_i^{\OL, \ell_p}(\dedup(A))
\end{align*}
thus showing that $\zeta_i$ is not too large compared to the online sensitivity of the $i$-th row with respect to $\dedup(A_{1:i})$.
